# Supplementary material for: Fragility of local moments against hybridization with flat bands
Source: arXiv:2503.14326 source file (2026-08-11)
Supplement: Supplementary file 1 [file Supplementary_material.tex]

\NeedsTeXFormat{LaTeX2e}
\documentclass[onecolumn,prb,aps,footinbib,amsmath,amssymb,superscriptaddress,longbibliography]{revtex4-2}
\PassOptionsToPackage{dvipsnames,svgnames,table}{xcolor}
\usepackage{xr}
\usepackage{array}
\usepackage{graphicx}
\usepackage{dcolumn}
\usepackage{color}
\usepackage{bm}
\usepackage{comment}
\usepackage{natbib}
\usepackage{tabularray}
\usepackage{multirow}
\usepackage{amsmath,amssymb,amsfonts,bbold}
\usepackage[normalem]{ulem}
\usepackage{nameref}
\usepackage{setspace}
\usepackage{float}
\usepackage{subfig}
\usepackage{physics}
\usepackage[justification=justified]{caption}
\usepackage{ragged2e}
% \captionsetup{justification=centering}

\externaldocument{main}

\usepackage[dvipsnames]{xcolor}

\usepackage[hidelinks]{hyperref}
\hypersetup{
  colorlinks   = true, %Colours links instead of ugly boxes
  urlcolor     = blue, %Colour for external hyperlinks
  linkcolor    = blue, %Colour of internal links
  citecolor   = blue %Colour of citations
}

\usepackage{booktabs}

%%%%%%%%%%%%%%%%%%%%%%%%%
% shorthands

\graphicspath{{fig/}}
 
\begin{document}

\title{Fragility of local moments against hybridization with flat bands}

\author{Max~Fischer}
\affiliation{Institut f{\"u}r Theoretische Physik und Astrophysik and W{\"u}rzburg-Dresden Cluster of Excellence ct.qmat, Universit{\"a}t W{\"u}rzburg, 97074 W{\"u}rzburg, Germany}

\author{Arianna~Poli} 
\affiliation{Dipartimento di Scienze Fisiche e Chimiche, Università dell'Aquila, Coppito-L'Aquila, Italy}

\author{Lorenzo~Crippa}
\affiliation{Institut f{\"u}r Theoretische Physik und Astrophysik and W{\"u}rzburg-Dresden Cluster of Excellence ct.qmat, Universit{\"a}t W{\"u}rzburg, 97074 W{\"u}rzburg, Germany}
\affiliation{I. Institute of Theoretical Physics, Universität Hamburg, Notkestraße 9-11, 22607 Hamburg, Germany}

\author{Dumitru~C\u{a}lug\u{a}ru}
\affiliation{Rudolf Peierls Centre for Theoretical Physics, University of Oxford, Oxford OX1 3PU, United Kingdom}

\author{Sergio~Ciuchi}
\affiliation{Dipartimento di Scienze Fisiche e Chimiche, Università dell'Aquila, Coppito-L'Aquila, Italy}

\author{Matthias~Vojta}
\affiliation{Institut für Theoretische Physik and W{\"u}rzburg-Dresden Cluster of Excellence ct.qmat, Technische Universit\"at Dresden, 01062 Dresden, Germany}

\author{Alessandro~Toschi}
\affiliation{Institute of Solid State Physics, TU Wien, 1040 Vienna, Austria}

\author{Giorgio~Sangiovanni}
\affiliation{Institut f{\"u}r Theoretische Physik und Astrophysik and W{\"u}rzburg-Dresden Cluster of Excellence ct.qmat, Universit{\"a}t W{\"u}rzburg, 97074 W{\"u}rzburg, Germany}

\date{\today}
\maketitle

\noindent
\section{Supplementary material}

\subsection{Anderson impurity model and hybridization function}
\label{sec:system_Hamiltonian_hyb_func_expansion_low_freq}
\noindent We start with the general form of a single-site Anderson impurity model:
\begin{equation}
   \hat{H}\,=\,\sum_{k,\,\sigma}\,\epsilon_{k}\,\hat{c}^{\dagger}_{k\sigma}\,\hat{c}_{k\sigma}\,+\,\sum_{\sigma}\,\epsilon_{f}\,\hat{f}^{\dagger}_{\sigma}\,\hat{f}_{\sigma}\,+\,U\,\hat{n}_{f\uparrow}\,\hat{n}_{f\downarrow}\,+\,\sum_{k,\,\sigma}\,V_k\,\left(\hat{c}^{\dagger}_{k\sigma}\,\hat{f}_{\sigma}\,+\,\hat{f}^{\dagger}_{\sigma}\,\hat{c}_{k\sigma}\right)\,,
\label{eq:general_AIM_Hamiltonian}
\end{equation}
where the first term describes the dispersion $\epsilon_{k}$ of the bath while the second and third terms are the energy level $\epsilon_{f}$ and the interaction $U$ on the impurity site, respectively. The last term denotes the hybridization between the bath and the impurity with the hybridization strength $V_k$, assumed to be constant within the scope of this paper ($V_k\,=\,V$). $\hat{f}^{(\dagger)}_{\sigma}$ and $\hat{c}^{(\dagger)}_{k\sigma}$ are annihilation (creation) operators on the impurity site and in the bath, respectively. The hybridization function is related to the retarded non-interacting Green's function $G_0(\omega)$ via
\begin{equation}
    \Delta(\omega)= \omega + i\eta - \epsilon_f - G^{-1}_0(\omega),
    \label{eq:G0}
\end{equation}
where $\eta$ denotes the symbol used to indicate 0$^+$.\\
For the hybridization function in the main text, we assumed half-filling and particle-hole symmetry, implying in this case $\epsilon_f = -\frac{U}{2}$.
\subsection{Hybridization function of a three-dimensional Dirac semimetal}
\noindent In the following we describe the procedure to calculate the hybridization function for one orbital, at half-filling with particle-hole symmetry at small frequencies for a 3D Dirac semimetal with energy cutoff $\mathcal{D}$. In this case the dispersion reads $\epsilon_{\vert{\mathbf{k}}\vert{}}\,=\,\vert{\mathbf{k}}\vert{}$ and the corresponding $-\frac{1}{\pi}\,\text{Im}\left[G_0(\epsilon)\right]$ becomes:
\begin{equation}
    -\frac{1}{\pi}\,\text{Im}\left[G_0(\epsilon)\right]\,\propto\,\int^{\infty}_{-\infty}\,\text{d}^3 \mathbf{k}\,\delta(\epsilon\,-\,\epsilon_{\vert{\mathbf{k}}\vert{}})\,\propto\,\int^{\infty}_{-\infty}\,\text{d} \vert{\mathbf{k}}\vert{}\,\vert{\mathbf{k}}\vert{}^2\,\delta(\epsilon\,-\,\vert{\mathbf{k}}\vert{})\,\propto\,\epsilon^2
\end{equation}
With the condition of a normalized $-\frac{1}{\pi}\,\text{Im}\left[G_0(\epsilon)\right]$, this yields:
\begin{equation}
    -\frac{1}{\pi}\,\text{Im}\left[G_0(\epsilon)\right]\,=\,\frac{3}{2\,\mathcal{D}^3}\,\epsilon^2
\end{equation}
\clearpage
\noindent
Using this result, we are able to calculate the non-interacting Green's function $G_0$:
\begin{equation}
    G_0(\omega)\,=\,\int^{\infty}_{-\infty}\,\text{d}\epsilon\,\frac{-\frac{1}{\pi}\,\text{Im}\left[G_0(\epsilon)\right]}{\omega\,+\,i\,\eta\,-\,\epsilon}\,=\,-\frac{3\,\left(\omega\,+\,i\,\eta\right)}{2\,\mathcal{D}^3}\,\left(2\,\mathcal{D}\,+\,\left(\omega\,+\,i\,\eta\right)\,\ln{\left(\frac{\omega\,+\,i\,\eta\,-\,\mathcal{D}}{\omega\,+\,i\,\eta\,+\,\mathcal{D}}\right)}\right)\,,
\end{equation}
where $\eta$ is a small imaginary part. If we compute the real and the imaginary part for the logarithm of the previous expression and take the limit where $\omega$ and $\eta$ are small, we get $\ln{\left(\frac{\omega\,+\,i\,\eta\,-\,\mathcal{D}}{\omega\,+\,i\,\eta\,+\,\mathcal{D}}\right)}\,\approx\,-i\,\frac{2\,\eta}{\mathcal{D}}\,+\,i\,\pi$ and find:
\begin{equation}
    G_0(\omega)\,=\,G'_0\,+\,i\,G''_0\,\approx\,-\frac{3}{\mathcal{D}^2}\,\left(1\,+\,\frac{\pi\,\eta}{\mathcal{D}}\right)\,\omega\,-\,i\,\frac{3}{\mathcal{D}^2}\,\left(\eta\,+\,\frac{\pi}{2\,\mathcal{D}}\,\omega^2\,-\,\frac{\pi}{2\,\mathcal{D}}\,\eta^2\right)\,.
\end{equation}
To determine the hybridization function we use the formula:
\begin{equation}
    \Delta(\omega)\,=\,\omega\,+\,i\,\eta\,-\,\left[G_0(\omega)\right]^{-1}\,=\,\frac{\omega\,\left(G'^2_0\,+\,G''^2_0\right)\,+\,i\,\eta\,\left(G'^2_0\,+\,G''^2_0\right)\,-\,G'_0\,+\,i\,G''_0}{G'^2_0\,+\,G''^2_0}\,,
\end{equation}
with $\mathcal{H}_\mathrm{loc}\,=\,0$. Inserting the previous approximations together with the limits $\eta\,\rightarrow{0}$ and $\omega\,\rightarrow{0}$ yields:
\begin{equation}
    -\frac{1}{\pi}\,\text{Im}\left[\Delta(\omega)\right]\,=\,-\frac{1}{\pi}\,\left[\eta\,+\,\frac{G''_0}{G'^2_0\,+\,G''^2_0}\right]\,\approx\,\frac{\mathcal{D}^2}{3}\,\delta(\omega)\,+\,\frac{\mathcal{D}}{6\,\pi}\,\frac{\left(\omega^2\,-\,\eta^2\right)}{\left(\omega^2\,+\,\eta^2\right)}\,\approx\,\frac{\mathcal{D}^2}{3}\,\delta(\omega)\,+\,\frac{\mathcal{D}}{6\,\pi}\,,
\end{equation}
describing a Dirac $\delta$-function together with a constant background.

\subsection{Impurity spin and charge susceptibilities}
\noindent
Two quantities we focus on in the main text are response functions on the impurity site for spin and charge. First, we define the $z$-spin susceptibility, quantifying the response of the system to an applied spin in $z$-direction. By using the particle number operators $n_i(\tau)$ in imaginary times $\tau$, we get the expression: 
\begin{equation}
    \chi_{zz}^{\text{spin}}(T)\,=\,g^2\,\int^\beta_0\,\text{d}\,\tau\,\big<\hat{S}_z(\tau)\,\hat{S}_z(0)\big>\,,
\label{eq:chi_spin_impurity_tau_integration}
\end{equation}
with ${\hat{S}_z(\tau)\,=\,\frac{1}{2}\,\left(n_{\uparrow}(\tau)\,-\,n_{\downarrow}(\tau)\right)}$ being the operator for the net spin in $z$-direction. The Lande factor $g$ is assumed to be 2 for electrons, and $\beta\,=\,\frac{1}{T}$ denotes the inverse temperature.\\
\noindent The charge susceptibility calculates the response of the system to double occupation on the impurity, such that an additional interaction $U$ applies. Here, the corresponding relation in terms of the number operators reads:
\begin{equation}
    \chi^{\text{charge}}(T)\,=\,\int_{0}^\beta\,\text{d}\tau\,\left<\left(\hat{n}_{\uparrow}(\tau)+\hat{n}_{\downarrow}(\tau)\right)\left(\hat{n}_{\uparrow}(0)+\hat{n}_{\downarrow}(0)\right)\right>\,-\,\beta\,\left<\left(\hat{n}_{\uparrow}+\hat{n}_{\downarrow}\right)\right>^2\,,
\end{equation}
where we already performed the $\tau$-integration in the second part.

\subsection{Analytic results for the spin and charge responses of a Kondo dimer at half-filling}
\label{sec:Analytic_results_Kondo_dimer_spin_charge_sus}
\noindent To construct a Kondo dimer, we assume a general Anderson impurity model with a single hybridization level and one impurity site:
\begin{equation}
   \hat{H}\,=\,\sum_{\sigma}\,\epsilon_{d}\,\hat{d}^{\dagger}_{\sigma}\,\hat{d}_{\sigma}\,+\,\sum_{\sigma}\,\epsilon_{f}\,\hat{f}^{\dagger}_{\sigma}\,\hat{f}_{\sigma}\,+\,V\,\sum_{\sigma}\,\left(\hat{d}^{\dagger}_{\sigma}\,\hat{f}_{\sigma}\,+\,\hat{f}^{\dagger}_{\sigma}\,\hat{d}_{\sigma}\right)\,+\,U\,\hat{n}_{f\uparrow}\,\hat{n}_{f\downarrow}\,,
\label{eq:AIM_Hamiltonian}
\end{equation}
with $d$ denoting quantities on the bath level and $f$ describing the impurity level. At half-filling the energy of the two levels are set to $\epsilon_f\,=\,-\frac{U}{2}$ and $\epsilon_d\,=\,0$, such that the Hamiltonian can be rewritten in the form:
\begin{equation}
    \hat{H}\,=\,U\,\hat{n}_{f\uparrow}\,\hat{n}_{f\downarrow}\,-\,\frac{U}{2}\,\left(\hat{n}_{f\uparrow}\,+\,\hat{n}_{f\downarrow}\right)\,+\,V\,\sum_{\sigma}\,\left(\hat{d}^{\dagger}_{\sigma}\,\hat{f}_{\sigma}\,+\,\hat{f}^{\dagger}_{\sigma}\,\hat{d}_{\sigma}\right)\,.
\end{equation}
This system can be solved analytically for the eigenenergies, summarized in TABLE\,\ref{tab:Kondo_dimer_energy_levels} and plotted in Fig.\,\ref{fig:histogramm_energy_levels} for $U\,=\,0$ (blue) and $U\,=\,5.75$ (orange) at the hybridization $V\,=\,2$ with the corresponding degeneracies. The prefactors $N_{ii}$ describe normalization factors for the eigenstates. 
\begin{figure}
    \centering
    \includegraphics[width=0.59\textwidth]{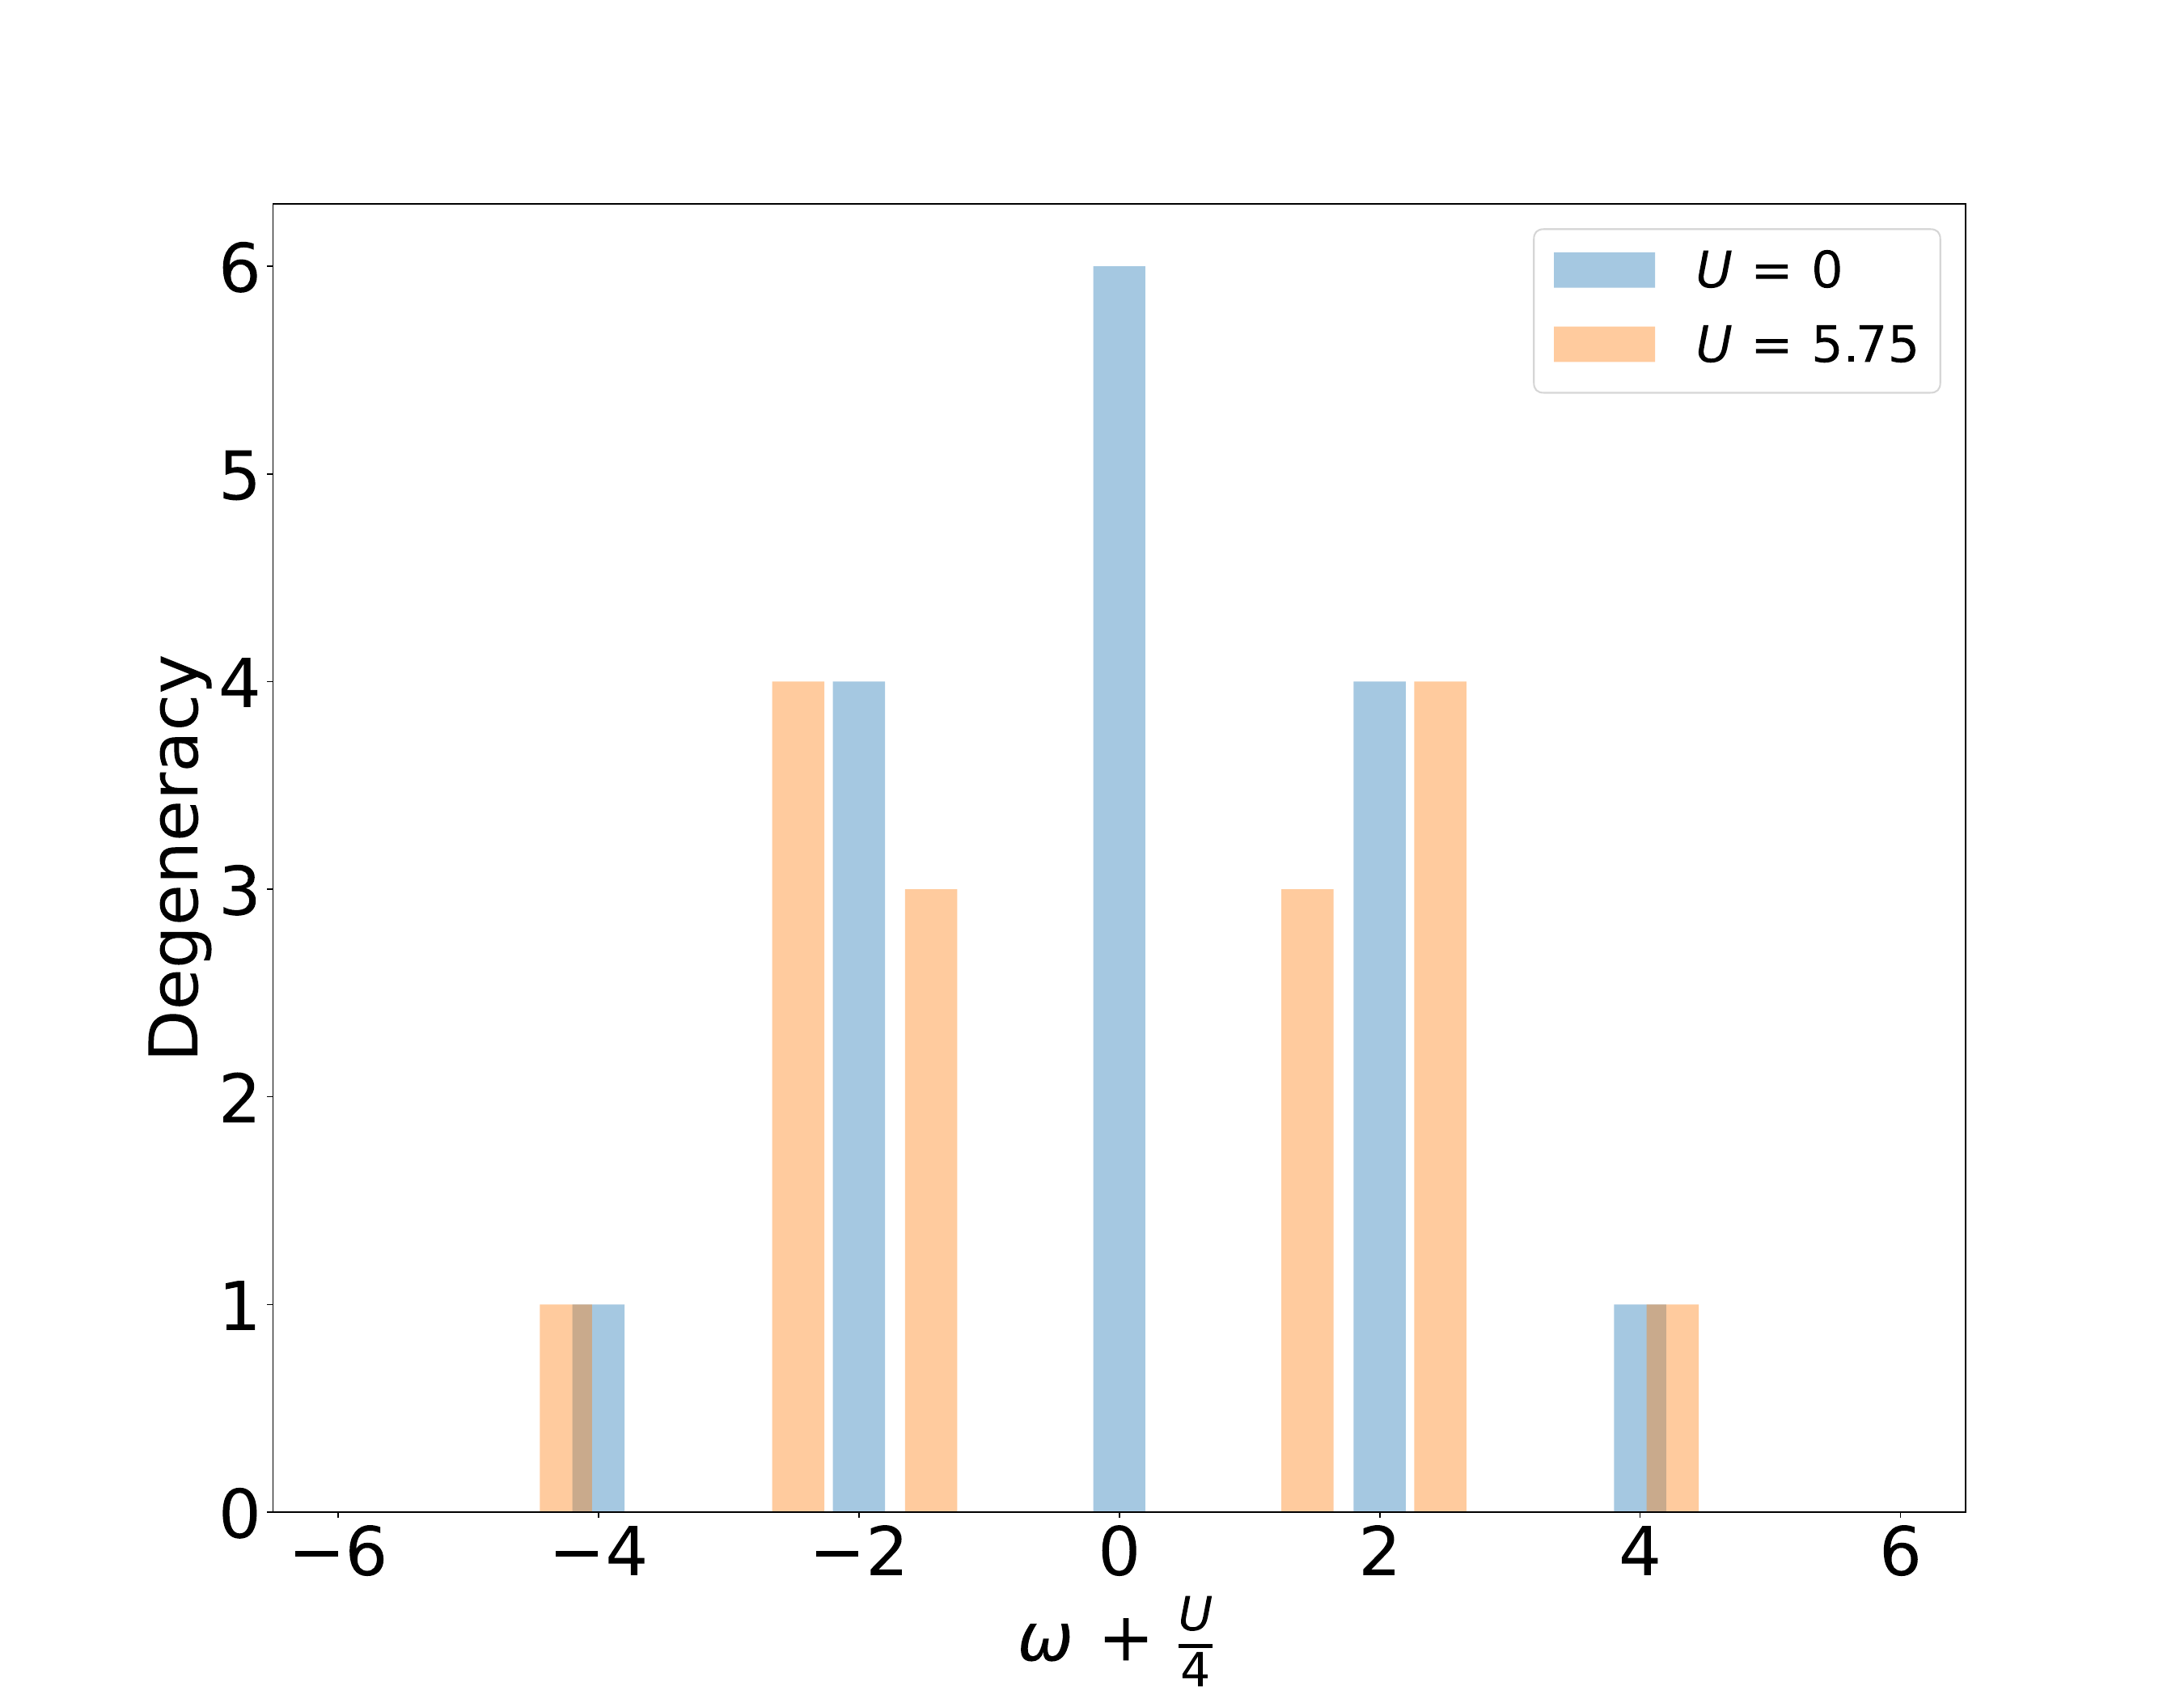}
    \caption{\justifying Energy levels of a Kondo dimer with one interacting site hybridized with a non-interacting site at half-filling with the interaction $U\,=\,0$ (blue) and $U\,=\,5.75$ (orange). Hopping between the sites is described by the hybridization $V\,=\,2$.}
    \label{fig:histogramm_energy_levels}
\end{figure}
With the eigenenergies we are able to establish the corresponding partition function:
\begin{equation}
    Z\,=\,\sum_n\,e^{-\beta\,\epsilon_n}\,=\,e^{-\beta\,\epsilon_0}\,+\,4\,e^{-\beta\,\epsilon_1}\,+\,3\,e^{-\beta\,\epsilon_2}\,+\,3\,e^{-\beta\,\epsilon_3}\,+\,4\,e^{-\beta\,\epsilon_4}\,+\,e^{-\beta\,\epsilon_5}\,,
\end{equation}
or by defining $\Delta_i\,=\,\epsilon_i\,-\,\epsilon_0$:
\begin{equation}
    Z\,=\,e^{-\beta\,\epsilon_0}\,\left(1\,+\,4\,e^{-\beta\,\Delta_1}\,+\,3\,e^{-\beta\,\Delta_2}\,+\,3\,e^{-\beta\,\Delta_3}\,+\,4\,e^{-\beta\,\Delta_4}\,+\,e^{-\beta\,\Delta_5}\right)\,.
\end{equation}

\begin{table*}
\SetTblrInner{rowsep=0.1cm}
\begin{tblr}{ ||p{5cm}|p{9.5cm}|p{1.2cm}||  }
 \hline
 % \multicolumn{3}{|c|}{Kondo dimer} \\
 \hline
 Energy levels & Eigenstates & Particles\\
 \hline
$\epsilon_0\,=\,-\frac{U}{4}\,-\,\sqrt{\left(\frac{U}{4}\right)^2\,+\,4\,V^2}$ & $\ket{n_{01}}\,=\,\frac{1}{N_{01}}\,\left(\epsilon_0\,\left(\ket{\uparrow,\,\downarrow}\,-\,\ket{\downarrow,\,\uparrow}\right)\,+\,2\,V\,\ket{2,\,0}\,+\,2\,V\,\ket{0,\,2}\right)$ & $n\,=\,2$\\
\hline

$\epsilon_1\,=\,-\frac{U}{4}\,-\,\sqrt{\left(\frac{U}{4}\right)^2\,+\,V^2}$ & $\ket{n_{11}}\,=\,\frac{1}{N_{11}}\,\left(\epsilon_1\,\ket{\uparrow,\,0}\,+\,V\,\ket{0,\,\uparrow}\right)$ & $n\,=\,1$\\
& $\ket{n_{12}}\,=\,\frac{1}{N_{12}}\,\left(\epsilon_1\,\ket{\downarrow,\,0}\,+\,V\,\ket{0,\,\downarrow}\right)$ & $n\,=\,1$\\
& $\ket{n_{13}}\,=\,\frac{1}{N_{13}}\,\left(\epsilon_1\,\ket{\uparrow,\,2}\,+\,V\,\ket{2,\,\uparrow}\right)$ & $n\,=\,3$\\
& $\ket{n_{14}}\,=\,\frac{1}{N_{14}}\,\left(\epsilon_1\,\ket{\downarrow,\,2}\,+\,V\,\ket{2,\,\downarrow}\right)$ & $n\,=\,3$\\
\hline

$\epsilon_2\,=\,-\frac{U}{2}$ & $\ket{n_{21}}\,=\,\frac{1}{N_{21}}\,\left(\ket{\uparrow,\,\downarrow}\,+\,\ket{\downarrow,\,\uparrow}\right)$ & $n\,=\,2$\\
& $\ket{n_{22}}\,=\,\ket{\uparrow,\,\uparrow}$ & $n\,=\,2$\\
& $\ket{n_{23}}\,=\,\ket{\downarrow,\,\downarrow}$ & $n\,=\,2$\\
\hline

$\epsilon_3\,=\,0$ & $\ket{n_{31}}\,=\,\frac{1}{N_{31}}\,\left(\ket{2,\,0}\,-\,\ket{0,\,2}\right)$ & $n\,=\,2$\\
& $\ket{n_{32}}\,=\,\ket{0,\,0}$ & $n\,=\,0$\\
& $\ket{n_{33}}\,=\,\ket{2,\,2}$ & $n\,=\,4$\\
\hline

$\epsilon_4\,=\,-\frac{U}{4}\,+\,\sqrt{\left(\frac{U}{4}\right)^2\,+\,V^2}$ & $\ket{n_{41}}\,=\,\frac{1}{N_{41}}\,\left(\epsilon_4\,\ket{\uparrow,\,0}\,+\,V\,\ket{0,\,\uparrow}\right)$ & $n\,=\,1$\\
& $\ket{n_{42}}\,=\,\frac{1}{N_{42}}\,\left(\epsilon_4\,\ket{\downarrow,\,0}\,+\,V\,\ket{0,\,\downarrow}\right)$ & $n\,=\,1$\\
& $\ket{n_{43}}\,=\,\frac{1}{N_{43}}\,\left(\epsilon_4\,\ket{\uparrow,\,2}\,+\,V\,\ket{2,\,\uparrow}\right)$ & $n\,=\,3$\\
& $\ket{n_{44}}\,=\,\frac{1}{N_{44}}\,\left(\epsilon_4\,\ket{\downarrow,\,2}\,+\,V\,\ket{2,\,\downarrow}\right)$ & $n\,=\,3$\\
\hline

$\epsilon_5\,=\,-\frac{U}{4}\,+\,\sqrt{\left(\frac{U}{4}\right)^2\,+\,4\,V^2}$ & $\ket{n_{51}}\,=\,\frac{1}{N_{51}}\,\left(\epsilon_5\,\left(\ket{\uparrow,\,\downarrow}\,-\,\ket{\downarrow,\,\uparrow}\right)\,+\,2\,V\,\ket{2,\,0}\,+\,2\,V\,\ket{0,\,2}\right)$ & $n\,=\,2$\\
\hline
\hline
\end{tblr}
\centering
\caption{\justifying Energy levels of a Kondo dimer (system with one interacting site hybridized with one non-interacting site) at half-filling. $N_{ii}$ describes a normalization constant for the respective eigenstates.}
\label{tab:Kondo_dimer_energy_levels}
\end{table*} 
\noindent For analytic calculations of spin and charge susceptibilities we use the Lehmann representation. Here, we differentiate transitions between different energy levels and contributions at the same energy. Starting with the spin susceptibility we find the following expression for transitions with varying energies:
\begin{equation}
\begin{split}
    \chi^{\text{spin},\,\epsilon_n\,\neq\,\epsilon_{n'}}_{zz}\,&=\,-\,\frac{1}{Z}\,\sum_{n\,\neq\,n'}\,\frac{e^{-\epsilon_n\,\beta\,}-\,e^{-\epsilon_{n'}\,\beta}}{\epsilon_n\,-\,\epsilon_{n'}}\,\vert{C_{n,\,n'}}\vert{}^2\\
    &=\,-\,\frac{1}{Z}\,e^{-\epsilon_0\,\beta}\,\frac{1\,-\,e^{-\Delta_2\,\beta}}{\Delta_2}\,\left(\vert{C_{0,\,2}}\vert{}^2\,+\,\vert{C_{2,\,0}}\vert{}^2\right)\,-\,\frac{1}{Z}\,e^{-\epsilon_0\,\beta}\,\frac{e^{-\Delta_1\,\beta}\,-\,e^{-\Delta_4\,\beta}}{\Delta_1\,-\,\Delta_4}\,\left(\vert{C_{1,\,4}}\vert{}^2\,+\,\vert{C_{4,\,1}}\vert{}^2\right)\\
    &\,\,\,\,\,\,\,-\,\frac{1}{Z}\,e^{-\epsilon_0\,\beta}\,\frac{e^{-\Delta_2\,\beta}\,-\,e^{-\Delta_5\,\beta}}{\Delta_2\,-\,\Delta_5}\,\left(\vert{C_{2,\,5}}\vert{}^2\,+\,\vert{C_{5,\,2}}\vert{}^2\right)\,,
\end{split}
\end{equation}
with $C_{n,\,n'}\,=\,\sum_i\,\bra{n_{n,\,i}}(\hat{n}_{f\uparrow}\,-\,\hat{n}_{f\downarrow})\ket{n_{n',\,i}}$, where $i$ indicates a sum over the eigenfunctions of the corresponding subspace for the respective energy.
\newpage
\noindent
If the energy levels are equal, we get:
\begin{equation}
\begin{split}
    \chi^{\text{spin},\,\epsilon_n\,=\,\epsilon_{n'}}_{zz}\,&=\,\frac{1}{Z}\,\sum_{n\,=\,n',\,j}\,\beta\,e^{-\epsilon_n\,\beta}\,\vert{C_{n, j}}\vert{}^2\\
    &=\,\frac{\beta}{Z}\,e^{-\epsilon_0\,\beta}\,e^{-\Delta_1\,\beta}\,\left(\vert{C_{1,\,1}}\vert{}^2\,+\,\vert{C_{1,\,2}}\vert{}^2+\,\vert{C_{1,\,3}}\vert{}^2\,+\,\vert{C_{1,\,4}}\vert{}^2\right)\,+\,\frac{\beta}{Z}\,e^{-\epsilon_0\,\beta}\,e^{-\Delta_2\,\beta}\,\left(\vert{C_{2,\,2}}\vert{}^2\,+\,\vert{C_{2,\,3}}\vert{}^2\right)\\
    &\,\,\,\,\,\,\,+\,\frac{\beta}{Z}\,e^{-\epsilon_0\,\beta}\,e^{-\Delta_4\,\beta}\,\left(\vert{C_{4,\,1}}\vert{}^2\,+\,\vert{C_{4,\,2}}\vert{}^2+\,\vert{C_{4,\,3}}\vert{}^2\,+\,\vert{C_{4,\,4}}\vert{}^2\right)\,,
\end{split}
\end{equation}
with $C_{n,\,j}\,=\,\bra{n_{n,\,j}}(\hat{n}_{f\uparrow}\,-\,\hat{n}_{f\downarrow})\ket{n_{n,\,j}}$.
The index $j$ refers to the $j$-th overlap at the same energy level. For $U\,=\,0$ and $V\,=\,2$ the previous expressions yield:
\begin{equation}
    \begin{split}
        \chi^{\text{spin},\,\epsilon_n\,\neq\,\epsilon_{n'}}_{zz}\,&=\,\frac{\frac{1}{2}\,+\,e^{-2\,\beta}\,-\,e^{-6\,\beta}\,-\,\frac{1}{2}\,e^{-8\,\beta}}{2\,\left[1\,+\,4\,e^{-2\,\beta}\,+\,6\,e^{-4\,\beta}\,+\,4\,e^{-6\,\beta}\,+\,e^{-8\,\beta}\right]}\\
        \chi^{\text{spin},\,\epsilon_n\,=\,\epsilon_{n'}}_{zz}\,&=\,\frac{\beta\,\left[e^{-2\,\beta}\,+\,2\,e^{-4\,\beta}\,+\,e^{-6\,\beta}\right]}{1\,+\,4\,e^{-2\,\beta}\,+\,6\,e^{-4\,\beta}\,+\,4\,e^{-6\,\beta}\,+\,e^{-8\,\beta}}
    \end{split}
\end{equation}
and the total spin susceptibility calculates to:
\begin{equation}
    \chi^{\text{spin}}_{zz}\,=\,\chi^{\text{spin},\,\epsilon_n\,\neq\,\epsilon_{n'}}_{zz}\,+\,\chi^{\text{spin},\,\epsilon_n\,=\,\epsilon_{n'}}_{zz}
\end{equation}
Focusing on the charge susceptibility and repeating the previous steps, we find the equations:
\begin{equation}
\begin{split}
    \chi^{\text{charge},\,\epsilon_n\,\neq\,\epsilon_{n'}}\,&=\,-\,\frac{1}{Z}\,\sum_{n\,\neq\,n'}\,\frac{e^{-\epsilon_n\,\beta\,}-\,e^{-\epsilon_{n'}\,\beta}}{\epsilon_n\,-\,\epsilon_{n'}}\,\vert{C_{n,\,n'}}\vert{}^2\\
    &=\,-\,\frac{1}{Z}\,e^{-\epsilon_0\,\beta}\,\frac{1\,-\,e^{-\Delta_3\,\beta}}{\Delta_3}\,\left(\vert{C_{0,\,3}}\vert{}^2\,+\,\vert{C_{3,\,0}}\vert{}^2\right)\,-\,\frac{1}{Z}\,e^{-\epsilon_0\,\beta}\,\frac{e^{-\Delta_1\,\beta}\,-\,e^{-\Delta_4\,\beta}}{\Delta_1\,-\,\Delta_4}\,\left(\vert{C_{1,\,4}}\vert{}^2\,+\,\vert{C_{4,\,1}}\vert{}^2\right)\\
    &\,\,\,\,\,\,\,-\,\frac{1}{Z}\,e^{-\epsilon_0\,\beta}\,\frac{e^{-\Delta_3\,\beta}\,-\,e^{-\Delta_5\,\beta}}{\Delta_3\,-\,\Delta_5}\,\left(\vert{C_{3,\,5}}\vert{}^2\,+\,\vert{C_{5,\,3}}\vert{}^2\right)
\end{split}
\end{equation}
and
\begin{equation}
\begin{split}
    \chi^{\text{charge},\,\epsilon_n\,=\,\epsilon_{n'}}\,&=\,\frac{1}{Z}\,\sum_{n\,=\,n',\,i}\,\beta\,e^{-\epsilon_n\,\beta}\,\vert{C_{n, i}}\vert{}^2\\
    &=\,\frac{\beta}{Z}\,e^{-\epsilon_0\,\beta}\,\vert{C_{0,\,1}}\vert{}^2\,+\,\frac{\beta}{Z}\,e^{-\epsilon_0\,\beta}\,e^{-\Delta_1\,\beta}\,\left(\vert{C_{1,\,1}}\vert{}^2\,+\,\vert{C_{1,\,2}}\vert{}^2+\,\vert{C_{1,\,3}}\vert{}^2+\,\vert{C_{1,\,4}}\vert{}^2\right)\\
    &\,\,\,\,\,\,\,+\,\frac{\beta}{Z}\,e^{-\epsilon_0\,\beta}\,e^{-\Delta_2\,\beta}\,\left(\vert{C_{2,\,1}}\vert{}^2\,+\,\vert{C_{2,\,2}}\vert{}^2\,+\,\vert{C_{2,\,3}}\vert{}^2\right)\,+\,\frac{\beta}{Z}\,e^{-\epsilon_0\,\beta}\,e^{-\Delta_3\,\beta}\,\left(\vert{C_{3,\,1}}\vert{}^2\,+\,\vert{C_{3,\,3}}\vert{}^2\right)\\
    &\,\,\,\,\,\,\,+\,\frac{1}{Z}\,e^{-\epsilon_0\,\beta}\,\beta\,e^{-\Delta_4\,\beta}\,\left(\vert{C_{4,\,1}}\vert{}^2\,+\,\vert{C_{4,\,2}}\vert{}^2+\,\vert{C_{4,\,3}}\vert{}^2\,+\,\vert{C_{4,\,4}}\vert{}^2\right)\,+\,\frac{\beta}{Z}\,e^{-\epsilon_0\,\beta}\,e^{-\Delta_5\,\beta}\,\vert{C_{5,\,1}}\vert{}^2\,.
\end{split}
\end{equation}
In the case of the local charge susceptibility there exists a non-vanishing disconnected part subtracted from the two other contributions in contrast to the local spin susceptibility:
\begin{equation}
\begin{split}
    \chi^{\text{charge},\,\text{discon}}\,&=\,\frac{\beta}{Z^2}\,\left(\sum_{n\,=\,n',\,i}\,e^{-\epsilon_n\,\beta}\,C_{n, i}\right)^2\\
    &=\,\frac{\beta}{Z^2}\,\left[e^{-\epsilon_0\,\beta}\,C_{0,\,1}\,+\,e^{-\epsilon_0\,\beta}\,e^{-\Delta_1\,\beta}\,\left(C_{1,\,1}\,+\,C_{1,\,2}\,+\,C_{1,\,3}\,+\,C_{1,\,4}\right)\right.\\
    &\left.\,\,\,\,\,\,\,+\,e^{-\epsilon_0\,\beta}\,e^{-\Delta_2\,\beta}\,\left(C_{2,\,1}\,+\,C_{2,\,2}\,+\,C_{2,\,3}\right)\,+\,e^{-\epsilon_0\,\beta}\,e^{-\Delta_3\,\beta}\,\left(C_{3,\,1}\,+\,C_{3,\,3}\right)\right.\\
    &\left.\,\,\,\,\,\,\,+\,e^{-\epsilon_0\,\beta}\,e^{-\Delta_4\,\beta}\,\left(C_{4,\,1}\,+\,C_{4,\,2}\,+\,C_{4,\,3}\,+\,C_{4,\,4}\right)\,+\,e^{-\epsilon_0\,\beta}\,e^{-\Delta_5\,\beta}\,C_{5,\,1}\right]^2\,.
\end{split}
\end{equation}
For the charge susceptibility, the $C$ matrix elements are calculated the same way as for the spin susceptibility, but with the expectation values of the charge operator $\hat{n}_{f\uparrow}\,+\,\hat{n}_{f\downarrow}$. 
Here, inserting $U\,=\,0$ and $V\,=\,2$ leads to:
\begin{equation}
    \begin{split}
        \chi^{\text{charge},\,\epsilon_n\,\neq\,\epsilon_{n'}}\,&=\,\frac{\frac{1}{2}\,+\,e^{-2\,\beta}\,-\,e^{-6\,\beta}\,-\,\frac{1}{2}\,e^{-8\,\beta}}{2\,\left[1\,+\,4\,e^{-2\,\beta}\,+\,6\,e^{-4\,\beta}\,+\,4\,e^{-6\,\beta}\,+\,e^{-8\,\beta}\right]}\\
        \chi^{\text{charge},\,\epsilon_n\,=\,\epsilon_{n'}}\,&=\,\frac{\beta\,\left[1\,+\,5\,e^{-2\,\beta}\,+\,8\,e^{-4\,\beta}\,+\,5\,e^{-6\,\beta}\,+\,e^{-8\,\beta}\right]}{1\,+\,4\,e^{-2\,\beta}\,+\,6\,e^{-4\,\beta}\,+\,4\,e^{-6\,\beta}\,+\,e^{-8\,\beta}}\\
        \chi^{\text{charge},\,\text{discon}}\,&=\,\frac{\beta\,\left[1\,+\,4\,e^{-2\,\beta}\,+\,6\,e^{-4\,\beta}\,+\,4\,e^{-6\,\beta}\,+\,e^{-8\,\beta}\right]}{1\,+\,4\,e^{-2\,\beta}\,+\,6\,e^{-4\,\beta}\,+\,4\,e^{-6\,\beta}\,+\,e^{-8\,\beta}}\,=\,\beta
    \end{split}
\end{equation}
and the total charge susceptibility consists of the following combination:
\begin{equation}
    \chi^{\text{charge}}\,=\,\chi^{\text{charge},\,\epsilon_n\,\neq\,\epsilon_{n'}}\,+\,\chi^{\text{charge},\,\epsilon_n\,=\,\epsilon_{n'}}\,-\,\chi^{\text{charge},\,\text{discon}}
\end{equation}
Thus, for $U\,=\,0$ and $V\,=\,2$ the charge and spin susceptibilities match each other.\\ In the following we analyze the limits of small and large temperatures for the local spin susceptibility.
\newpage
\subsubsection{Local spin susceptibility for $T\rightarrow{0}$}
\noindent
In the case $T\,\rightarrow{0}$, the exponential functions vanish and only a constant part in $T$ survives:
\begin{equation}
    \chi^{\text{spin}}_{zz}(T\,\rightarrow{0})\,=\,\chi^{\text{spin},\,\epsilon_n\,\neq\,\epsilon_{n'}}_{zz}(T\,\rightarrow{0})\,=\,\frac{\left(\vert{C_{0,\,2}}\vert{}^2\,+\,\vert{C_{2,\,0}}\vert{}^2\right)}{\Delta_2}\,=\,\frac{4\,\epsilon^2_0}{\epsilon_5\,\left(2\,\epsilon^2_0\,+\,8\,V^2\right)}\,=\,const.\,,
\end{equation}
depending on the interaction $U$, the hybridization $V$ and the eigenenergies summarized in TABLE\,\ref{tab:Kondo_dimer_energy_levels}.

\subsubsection{Large temperature limit}
\noindent
At high temperatures the zeroth order in the expansion around $\beta\,=\,0$ vanishes and only the first order in $\beta$ contributes to the local spin susceptibility:
\begin{equation}
\begin{split}
    \chi^{\text{spin}}_{zz}(T\,\rightarrow{\infty})\,=\,\frac{\beta}{2}\,,
\end{split}
\end{equation}
showing a Curie law for the Kondo dimer at large temperatures.

\subsection{Limit of high temperature and large interaction for the effective moment}
\noindent In the infinite temperature limit $T\,\rightarrow{\infty}$ all eigenstates $|\,i\big>$ of a system are equally distributed following the Boltzmann distribution: ${e^{-\beta\,\epsilon_i}\,=\,1\,\,\,\,\forall\,\epsilon_i}$, with the eigenenergies $\epsilon_i$. We begin with the definition of the expectation value for the squared $z$-spin operator $\big<\hat{S}^2_z\big>$:
\begin{equation}
    \big<\hat{S}^2_z\big>\,=\,\frac{1}{Z}\,\sum_{i}\,e^{-\beta\,\epsilon_i}\,\big<i\,|\hat{S}^2_z|\,i\big>.
\end{equation}
The corresponding partition function $Z$ reads:
\begin{equation}
    Z\,=\,\sum_{i}\,1\,=\,2^{2\,N_{\text{orb}}}\,,
\end{equation}
with the number of orbitals on the impurity site $N_{\text{orb}}$. Using the representation $\hat{S}_z\,=\,\frac{\hat{n}_{\uparrow}\,-\,\hat{n}_{\downarrow}}{2}$ for the $z$-spin operator, with $n_\uparrow$ the number of spin-up and $n_\downarrow$ the number of spin-down electrons and taking into account all possibilities for up and down electrons on the impurity site, we get the following representation:
\begin{equation}
    \sum_{i}\big<i\,|\hat{S}^2_z|\,i\big>=\frac{1}{4}\sum^{N_{\text{orb}}}_{n_\uparrow,n_\downarrow=0}\binom{N_{\text{orb}}}{n_\uparrow}\binom{N_{\text{orb}}}{n_\downarrow}\left(n_\uparrow-n_\downarrow\right)^2\,=\,2^{(2\,N_{\text{orb}}\,-\,1)}\,\frac{N_{\text{orb}}}{4}\,=\,2^{(2\,N_{\text{orb}}\,-\,3)}\,N_{\text{orb}}
\end{equation}
and for the expectation value of the squared spin-$z$ operator:
\begin{equation}
    \big<\hat{S}^2_z\big>(T\,\rightarrow{\infty})\,=\,\frac{1}{Z}\,\left(2^{(2\,N_{\text{orb}}\,-\,3)}\,N_{\text{orb}}\right)\,=\,\frac{N_{\text{orb}}}{8}\,.
\end{equation}
Thus, the overall local spin susceptibility has the form:
\begin{equation}
    \chi^{\text{spin}}_{\text{zz}}(T\,\rightarrow{\infty})\,=\,\frac{g^2\,\big<\hat{S}^2_z\big>}{T}\,=\,\frac{N_{\text{orb}}}{2\,T}\,.
\end{equation}
\newpage
\noindent
Comparing this with a Curie behavior including an effective moment $\mu_\text{eff}$:
\begin{equation}
    \chi^{\text{spin}}_{\text{zz}}\,=\,\frac{\mu^2_\text{eff}}{3\,T}\,,
\end{equation}
yields:
\begin{equation}
    \mu_\text{eff}(T\,\rightarrow{\infty})\,=\,\sqrt{\frac{3\,N_\text{orb}}{2}}\,.
\end{equation}
\noindent For the atomic limit ($U\,\rightarrow{\infty}$) we write the squared $z$-spin operator $\big<\hat{S}^2_z\big>$ as:
\begin{equation}
    \big<\hat{S}^2_z\big>\,=\,\frac{\big<\left(\hat{n}_\uparrow\,-\,\hat{n}_\downarrow\right)^2\big>}{2}\,\approx\,\frac{\big<\hat{n}_\uparrow\big>\,+\,\big<\hat{n}_\downarrow\big>}{2}\,,
\end{equation}
since the expectation value for double occupation is zero. Furthermore, the single occupation has the value $\frac{1}{2}$ ($\frac{1}{4}$ for both spin-species), such that $\big<\hat{n}_\uparrow\big>\,=\,\big<\hat{n}_\downarrow\big>\,=\,\frac{N_\text{orb}}{4}$ leads to:
\begin{equation}
    \big<\hat{S}^2_z\big>(U\,\rightarrow{\infty})\,=\,\frac{N_\text{orb}}{4}\,.
\end{equation}
Following the same arguments as in the high temperature calculation, we find:
\begin{equation}
    \mu_\text{eff}(U\,\rightarrow{\infty})\,=\,\sqrt{3\,N_\text{orb}}\,.
\end{equation}

\subsection{High temperature expansion for the effective moment}
\noindent To investigate the large temperature expansion of the effective moment $\mu_\text{eff}$ we assume the Hamiltonian for the Kondo dimer in Eq.(\ref{eq:AIM_Hamiltonian}) perturbed by an external magnetic field $h$:
\begin{equation}
    \hat{H}_\text{perturbed}\,=\,\hat{H}\,-\,h\,\left(\hat{f}^\dagger_{\uparrow}\,\hat{f}_{\uparrow}\,-\,\hat{f}^\dagger_{\downarrow}\,\hat{f}_{\downarrow}\right)\,.
\end{equation}
Since the one- and three-particle subspaces have the highest contributions to the local spin susceptibility at large temperatures, we focus only on these cases. The Hamiltonian of the one- (three-) particle subspace reads:
\begin{equation}
\begin{split}
    \hat{H}_{1 (3)}\,&=\,\begin{pmatrix}0 && (-)V && 0 && 0\\ (-)V && \frac{U}{2}\,-\,h && 0 && 0\\ 0 && 0 && 0 && (-)V\\ 0 && 0 && (-)V && \frac{U}{2}\,+\,h\end{pmatrix}\\
    &=\begin{pmatrix}-\left(\frac{U}{4}\,+\,\frac{h}{2}\right)\,\mathbb{1}\,\pm\,V\,\sigma_x\,+\,\left(\frac{U}{4}\,+\,\frac{h}{2}\right)\,\sigma_z && 0\\ 0 && -\left(\frac{U}{4}\,-\,\frac{h}{2}\right)\,\mathbb{1}\,\pm\,V\,\sigma_x\,+\,\left(\frac{U}{4}\,-\,\frac{h}{2}\right)\,\sigma_z\end{pmatrix}\\
    &=\begin{pmatrix}n_0\,\mathbb{1}\,\pm\,n_1\,\sigma_x\,+\,n_3\,\sigma_z && 0\\ 0 && n'_0\,\mathbb{1}\,\pm\,n'_1\,\sigma_x\,+\,n'_3\,\sigma_z\end{pmatrix}\,,
\end{split}
\end{equation}
with the eigenvalues:
\begin{equation}
\begin{split}
        \epsilon_{1,\,2}\,&=\,-\left(\frac{U}{4}\,+\frac{h}{2}\right)\,\pm\,\sqrt{\left[\frac{U}{4}\,+\,\frac{h}{2}\right]^2\,+\,V^2}\,=\,n_0\,\pm\,\sqrt{n^2_1\,+\,n^2_3}\,=\,n_0\,\pm\,\vert{\mathbf{n}}\vert{}\\
        \epsilon_{3,\,4}\,&=\,-\left(\frac{U}{4}\,-\frac{h}{2}\right)\,\pm\,\sqrt{\left[\frac{U}{4}\,-\,\frac{h}{2}\right]^2\,+\,V^2}\,=\,n'_0\,\pm\,\sqrt{n'^2_1\,+\,n'^2_3}\,=\,n'_0\,\pm\,\vert{\mathbf{n}'}\vert{}\,.
\end{split}
\end{equation}
Here, we renamed the prefactors of the Pauli matrices as $\mathbf{n}^{(}{'^{)}}\,=\,\left(n_1{^{(}{'^{)}}},\,\,n_2{^{(}{'^{)}}},\,\,n_3{^{(}{'^{)}}}\right)^\text{T}$ and of the unity matrix as $n_0{^{(}{'^{)}}}$.
The partition functions of the two $2\times2$ matrix blocks are:
\begin{equation}
\begin{split}
    Z_{1 (3)}\,&=\,e^{-\beta\,\epsilon_1}\,+\,e^{-\beta\,\epsilon_2}\\
    Z'_{1 (3)}\,&=\,e^{-\beta\,\epsilon_3}\,+\,e^{-\beta\,\epsilon_4}\,.
\end{split}
\end{equation}
As next step we determine the magnetization in the canonical ensemble:
\begin{equation}
    M\,=\,\big<\,\hat{S}_z\,\big>\,=\,\frac{\text{Tr}\left[e^{-\beta\,\hat{H}_\text{perturbed}}\,\hat{S}_z\right]}{\text{Tr}\left[e^{-\beta\,\hat{H}_\text{perturbed}}\right]}\,,
\end{equation}
by introducing the $z$-spin operator $\hat{S}_z$:
\begin{equation}
    \hat{S}_z\,=\,\begin{pmatrix}0 && 0 && 0 && 0\\ 0 && 1 && 0 && 0\\ 0 && 0 && 0 && 0\\ 0 && 0 && 0 && -1\end{pmatrix}\,=\,\begin{pmatrix}\frac{1}{2}\,\mathbb{1}\,-\,\frac{1}{2}\,\sigma_z && 0\\ 0 && -\left(\frac{1}{2}\,\mathbb{1}\,-\,\frac{1}{2}\,\sigma_z\right)\end{pmatrix}\,.
\end{equation}
Using the properties of the Pauli matrices, the exponential in the magnetization can be written as:
\begin{equation}
    e^{-\beta\,\hat{H}^{2\times2}_\text{perturbed}}\,=\,e^{-\beta\,n_0{^{(}{'^{)}}}}\,\left(\cosh{\left(\beta\,\vert{\mathbf{n}^{(}{'^{)}}}\vert{}\right)}\,\mathbb{1}\,-\,\sinh{\left(\beta\,\vert{\mathbf{n}^{(}{'^{)}}}\vert{}\right)}\,\frac{\mathbf{n}^{(}{'^{)}}}{\vert{\mathbf{n}^{(}{'^{)}}}\vert{}}\,\cdot\,\boldsymbol{\sigma}\right)\,,
\end{equation}
for the respective $2\times2$-blocks and both subspaces.
\noindent With these expressions we are able to establish the overall magnetization in the one- and three-particle sectors:
\begin{equation}
    M_{1 (3)}\,=\,\frac{1}{Z_{1 (3)}\,+\,Z'_{1 (3)}}\,\left[e^{-\beta\,n_0}\,\left(\cosh{\left(\beta\,\vert{\mathbf{n}}\vert{}\right)}\,+\,\sinh{\left(\beta\,\vert{\mathbf{n}}\vert{}\right)\,\cdot\,\frac{n_3}{\vert{\mathbf{n}}\vert{}}}\right)\,-e^{-\beta\,n'_0}\,\left(\cosh{\left(\beta\,\vert{\mathbf{n}'}\vert{}\right)}\,+\,\sinh{\left(\beta\,\vert{\mathbf{n}'}\vert{}\right)\,\cdot\,\frac{n'_3}{\vert{\mathbf{n}'}\vert{}}}\right)\right]\,.
\end{equation}
Since we are interested in the limit of high temperatures, we expand the magnetization around $\beta\,=\,0$ up to second order:
\begin{equation}
    M_{1 (3)}(T\,\rightarrow{\infty})\,\approx\,\left[\frac{\beta}{4}\,\left(n_3-n_0-n'_3+n'_0\right)\,+\,\frac{\beta^2}{8}\,\left(\vert{\mathbf{n}}\vert{}^2\,-\,\vert{\mathbf{n}'}\vert{}^2\,-\,3\,n_0\,n_3\,+\,3\,n'_0\,n'_3\,+\,n_0\,n'_3\,-\,n_3\,n'_0\,+\,n^2_0\,-\,n'^2_0\right)\right]\,.
\end{equation}
Performing the derivative for the magnetic field $h$, we arrive at the high temperature expansion of the local spin susceptibility:
\begin{equation}
    \chi^{\text{spin}}_{zz}(T\,\rightarrow{\infty})\,=\,\frac{\partial M_{1 (3)}(T\,\rightarrow{\infty})}{\partial h}\,\approx\,\beta\,\left(\frac{1}{2}\,+\,\beta\,\frac{U}{8}\right)
\end{equation}
and with the definition $\mu_\text{eff}\,=\,\sqrt{3\,T\,\chi^{\text{spin}}_{zz}}$ we find the effective moment at high temperatures:
\begin{equation}
    \mu_\text{eff}(T\,\rightarrow{\infty})\,=\,\sqrt{\frac{3}{2}\left(1\,+\,\frac{U}{4\,T}\right)}\,\approx\,\sqrt{\frac{3}{2}}\,\left(1\,+\,\frac{U}{8\,T}\right)\,.
\end{equation}
This corresponds to the analytic results of section \ref{sec:Analytic_results_Kondo_dimer_spin_charge_sus} for large temperatures, but up to first order in $\beta$.\\
Fig.\,\ref{fig:Comparison_mu_eff_dif_V} shows the high temperature expansion for the effective moment (purple) together with curves of analytic results for a Kondo dimer at an interaction of $U\,=\,10\,\mathcal{D}$ for different values of the hybridization $V$. Increasing $V$ in relation to $U$, the effective moment $\mu_\text{eff}$ does no longer reach its maximum at the plateau $\mu_\text{eff}(U\,\rightarrow{\infty})\,=\,\sqrt{3}$, since the formation of a singlet ground state is favored.

\begin{figure}
    \centering
    \includegraphics[width=0.59\textwidth]{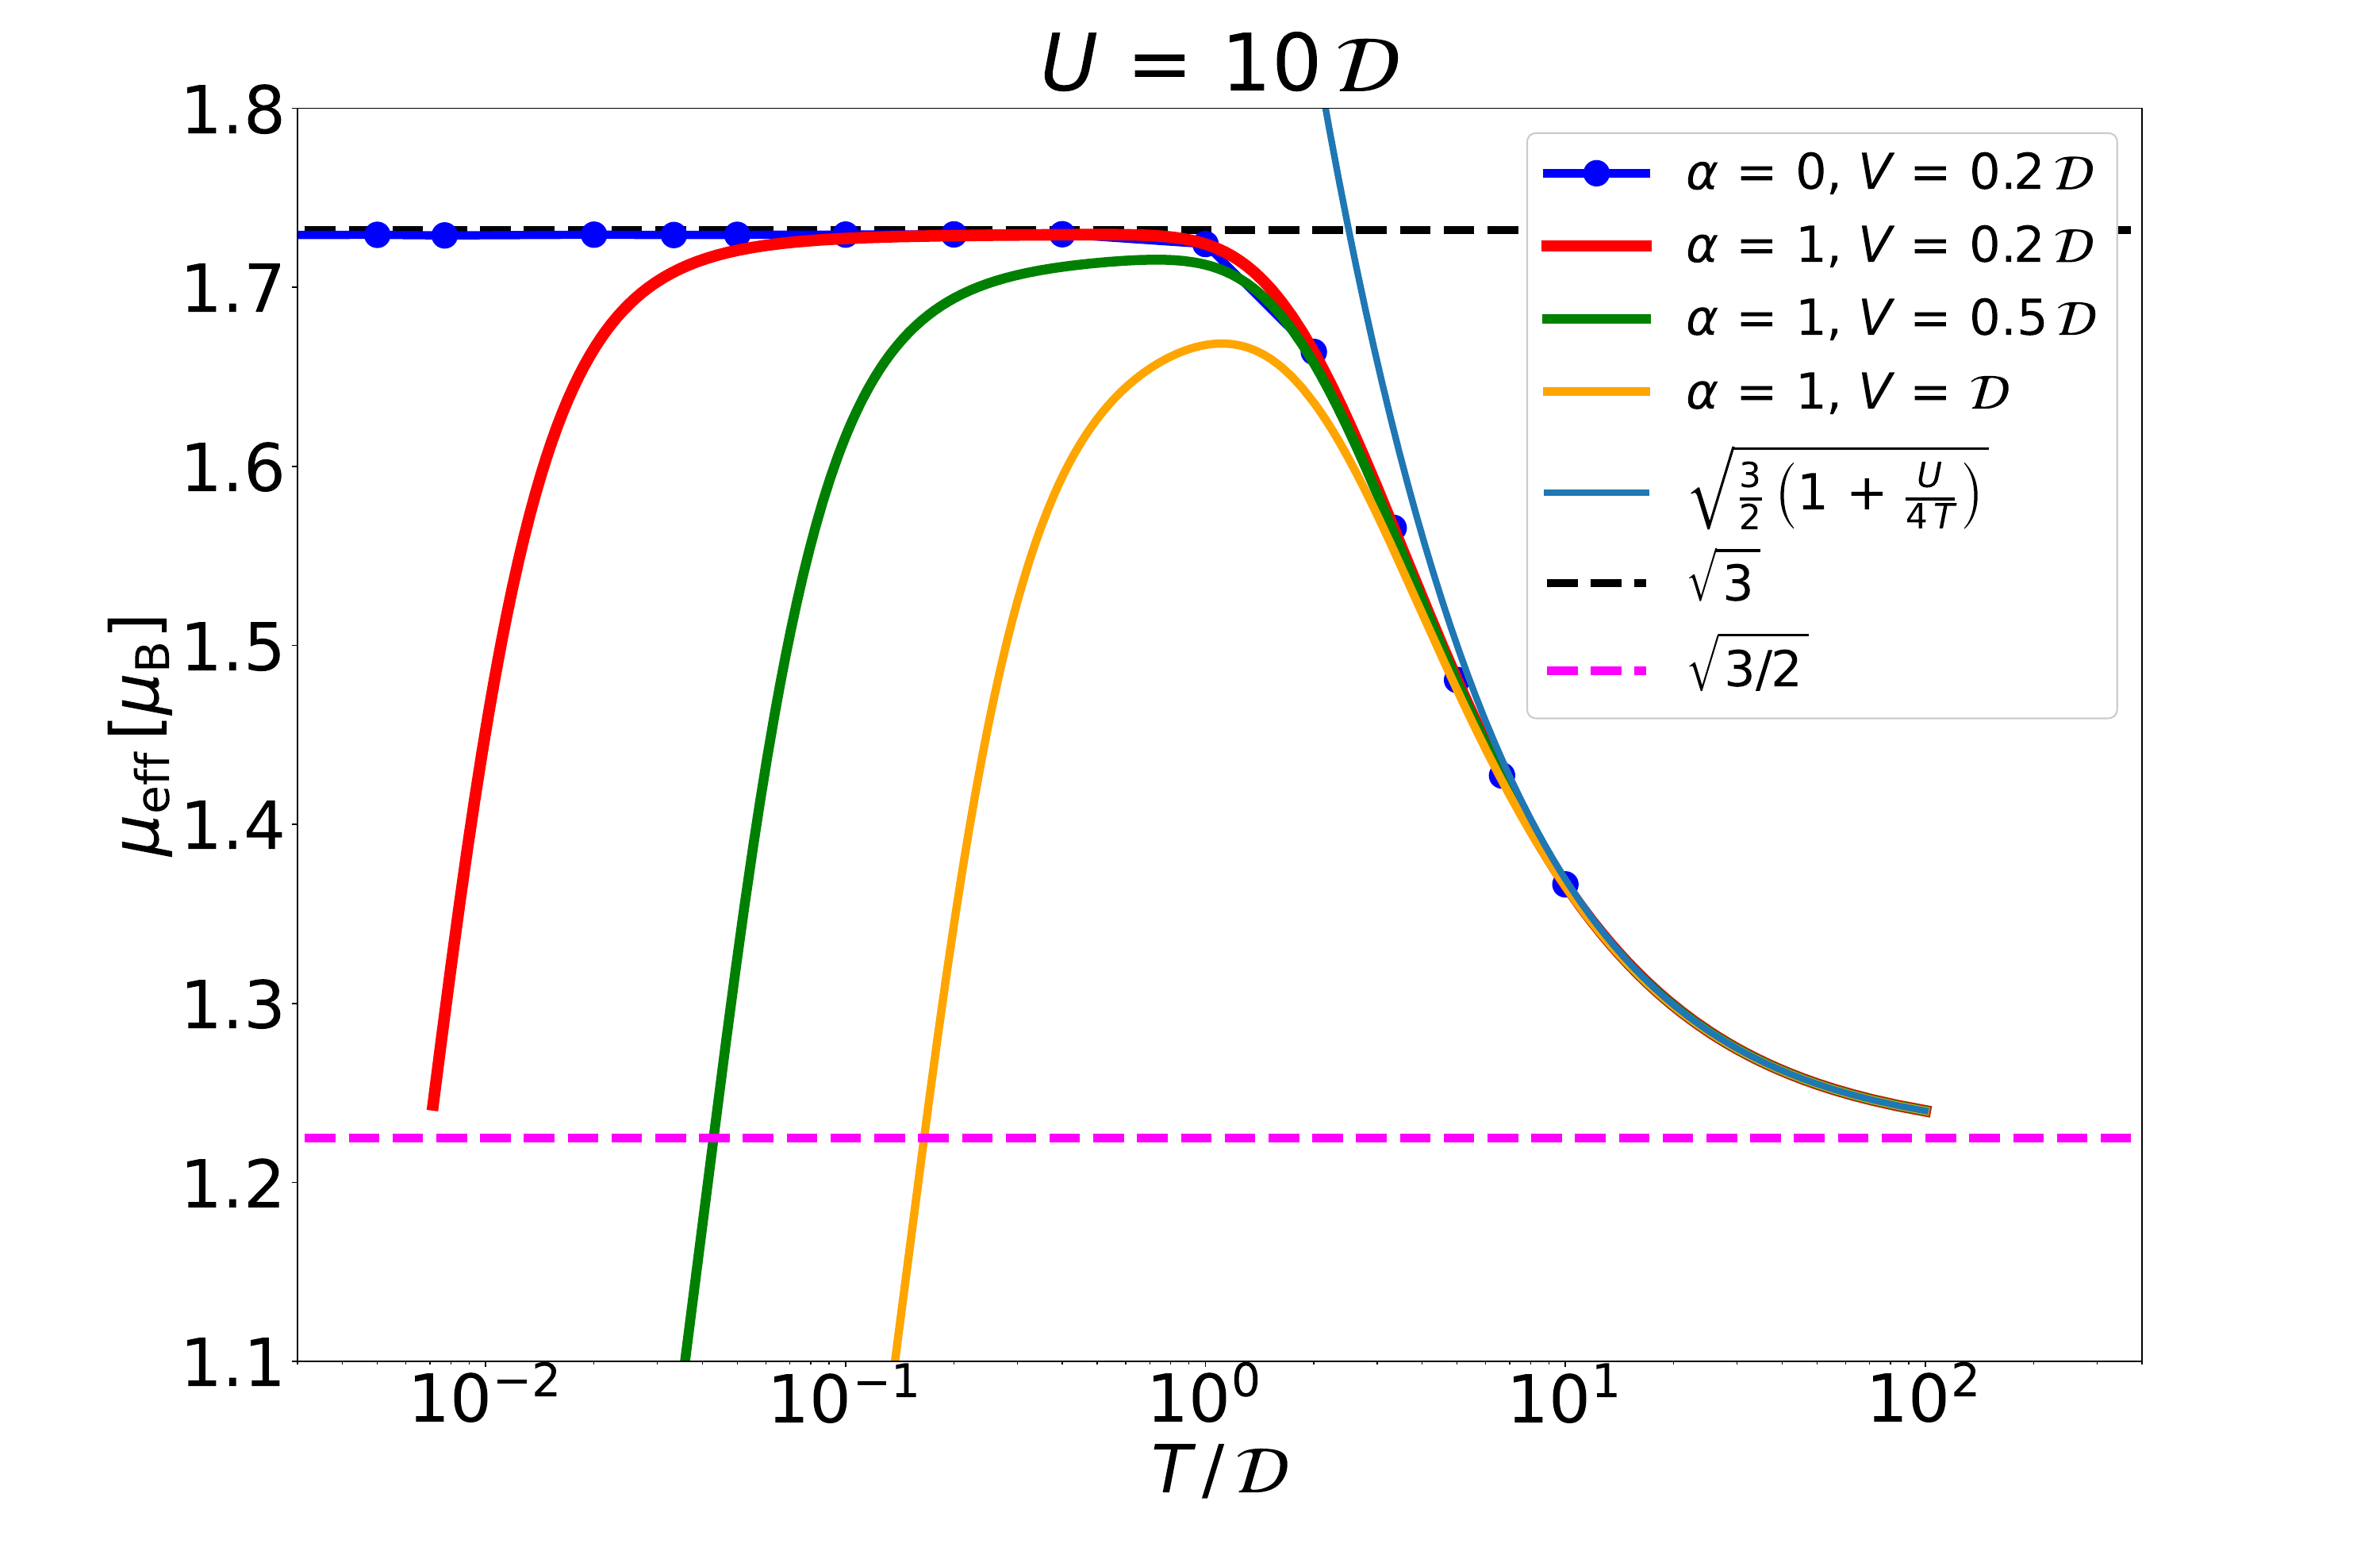}
    \caption{\justifying Comparison of the curves for analytic calculations of a Kondo dimer with interaction $U\,=\,10\,\mathcal{D}$ at several hybridizations ($V\,=\,0.2\,\mathcal{D}$ (red), $V\,=\,0.5\,\mathcal{D}$ (green), $V\,=\,\mathcal{D}$ (orange)). The plateau of the large $U$ limit for the effective moment is not reached at larger hybridizations. Purple: Large temperature expansion of analytic calculations within perturbation theory. Blue: $\mu_\text{eff}$ for a box-like hybridization function at $U\,=\,10\,\mathcal{D}$ and $V\,=\,0.2\,\mathcal{D}$. Here, the curve reaches the maximum effective moment over a long temperature range.}
    \label{fig:Comparison_mu_eff_dif_V}
\end{figure}
\newpage
\subsection{Scattering phase shift at $U\,=\,0$}
\noindent Following the calculations in \cite{Coleman_2015} for the scattering phase shift between the localized impurity fermion with the electron bath, we start with our Anderson impurity Hamiltonian Eq.\eqref{eq:general_AIM_Hamiltonian} for a single impurity site without interactions ($U\,=\,0$). The tunneling between the impurity and the bath is described by the hybridization function:
\begin{equation}
    \Delta(\omega)\,=\,\int^{\mathcal{D}}_\mathcal{-D}\,\text{d}\varepsilon\,\left[-\frac{1}{\pi}\,\frac{\text{Im}\left[\Delta(\varepsilon)\right]}{\omega\,-\,\varepsilon}\right]\,.
\end{equation}
As in the rest of this work, with $\mathcal{D}$ and $\mu$ we denote the frequency cutoff and the chemical potential, respectively while, with $\eta$ a small imaginary part. The retarded non-interacting impurity Green's function can then be written as
\begin{equation}
    G_0(\omega)\,=\,\frac{1}{\omega\,+\,i\,\eta \,-\,\epsilon_{f}\,-\,\Delta(\omega)}\,,
    \label{eq-suppl:Green}
\end{equation}
where $\epsilon_{f}$ is set to zero for the system under consideration. The corresponding density of states on the impurity reads:
\begin{equation}
    DOS(\omega)\,=\,-\,\frac{1}{\pi}\,\text{Im}\left[G_0(\omega)\right]\,.
    \label{eq-suppl:DOS}
\end{equation}
As next step, we use two different forms of the scattering T-matrix:\\
(i) Defining the $T$-matrix as bath electrons scattering at the impurity depending on the hybridization strength $V$ and moving back in the bath, it has the definition:
\begin{equation}
    T(\omega)\,=\,V^2\,G_0(\omega)\,.
\end{equation}
(ii) The second relation for the $T$-matrix comes from the $S$-matrix defined by the scattering phase shift $\xi(\omega)$ as:
\begin{equation}
    S(\omega)\,=\,e^{2\,i\,\xi(\omega)}\,.
\end{equation}
\newpage
\noindent
This $S$-matrix is connected to the $T$-matrix by the formula:
\begin{equation}
    S(\omega)\,=\,1\,-\,2\,\pi\,i\,\rho(\omega)\,T(\omega)\,,
\end{equation}
with $\rho(\omega)\,=\,-\frac{1}{\pi\,V^2}\,\text{Im}\left[\Delta(\omega)\right]$ being the density of states of the bath fermions. Solving these equations for the $T$-matrix yields:
\begin{equation}
    T(\omega)\,=\,-\frac{1}{\pi\,\rho(\omega)}\,\frac{1}{\cot{\left(\xi(\omega)\right)}\,-\,i}
\end{equation}
Comparing both expression for the $T$-matrix leads to the scattering phase shift depending on the hybridization function:
\begin{equation}
    \xi(\omega)\,=\,\text{arccot}\left(\frac{\omega\,-\,\text{Re}\left[\Delta(\omega)\right]}{\text{Im}\left[\Delta(\omega)\right]}\right)\,=\,\begin{cases} \text{arctan}\left(\frac{\text{Im}\left[\Delta(\omega)\right]}{\omega\,-\,\text{Re}\left[\Delta(\omega)\right]}\right),\quad \text{if} \quad \text{arg}(\text{arctan})\,\ge\,0 \\ \text{arctan}\left(\frac{\text{Im}\left[\Delta(\omega)\right]}{\omega\,-\,\text{Re}\left[\Delta(\omega)\right]}\right)\,+\,\pi,\quad \text{if} \quad \text{arg}(\text{arctan})\,<\,0\end{cases}\,.
\end{equation}
The scattering phase shift together with the impurity density of states is summarized in Fig.\,\ref{fig:scattering_phase_shift_and_impurity_DOS} (a) and (b) for the different weights of $\alpha$ discussed in the main text.
\begin{figure*}
    \centering
    \includegraphics[width=0.85\textwidth]{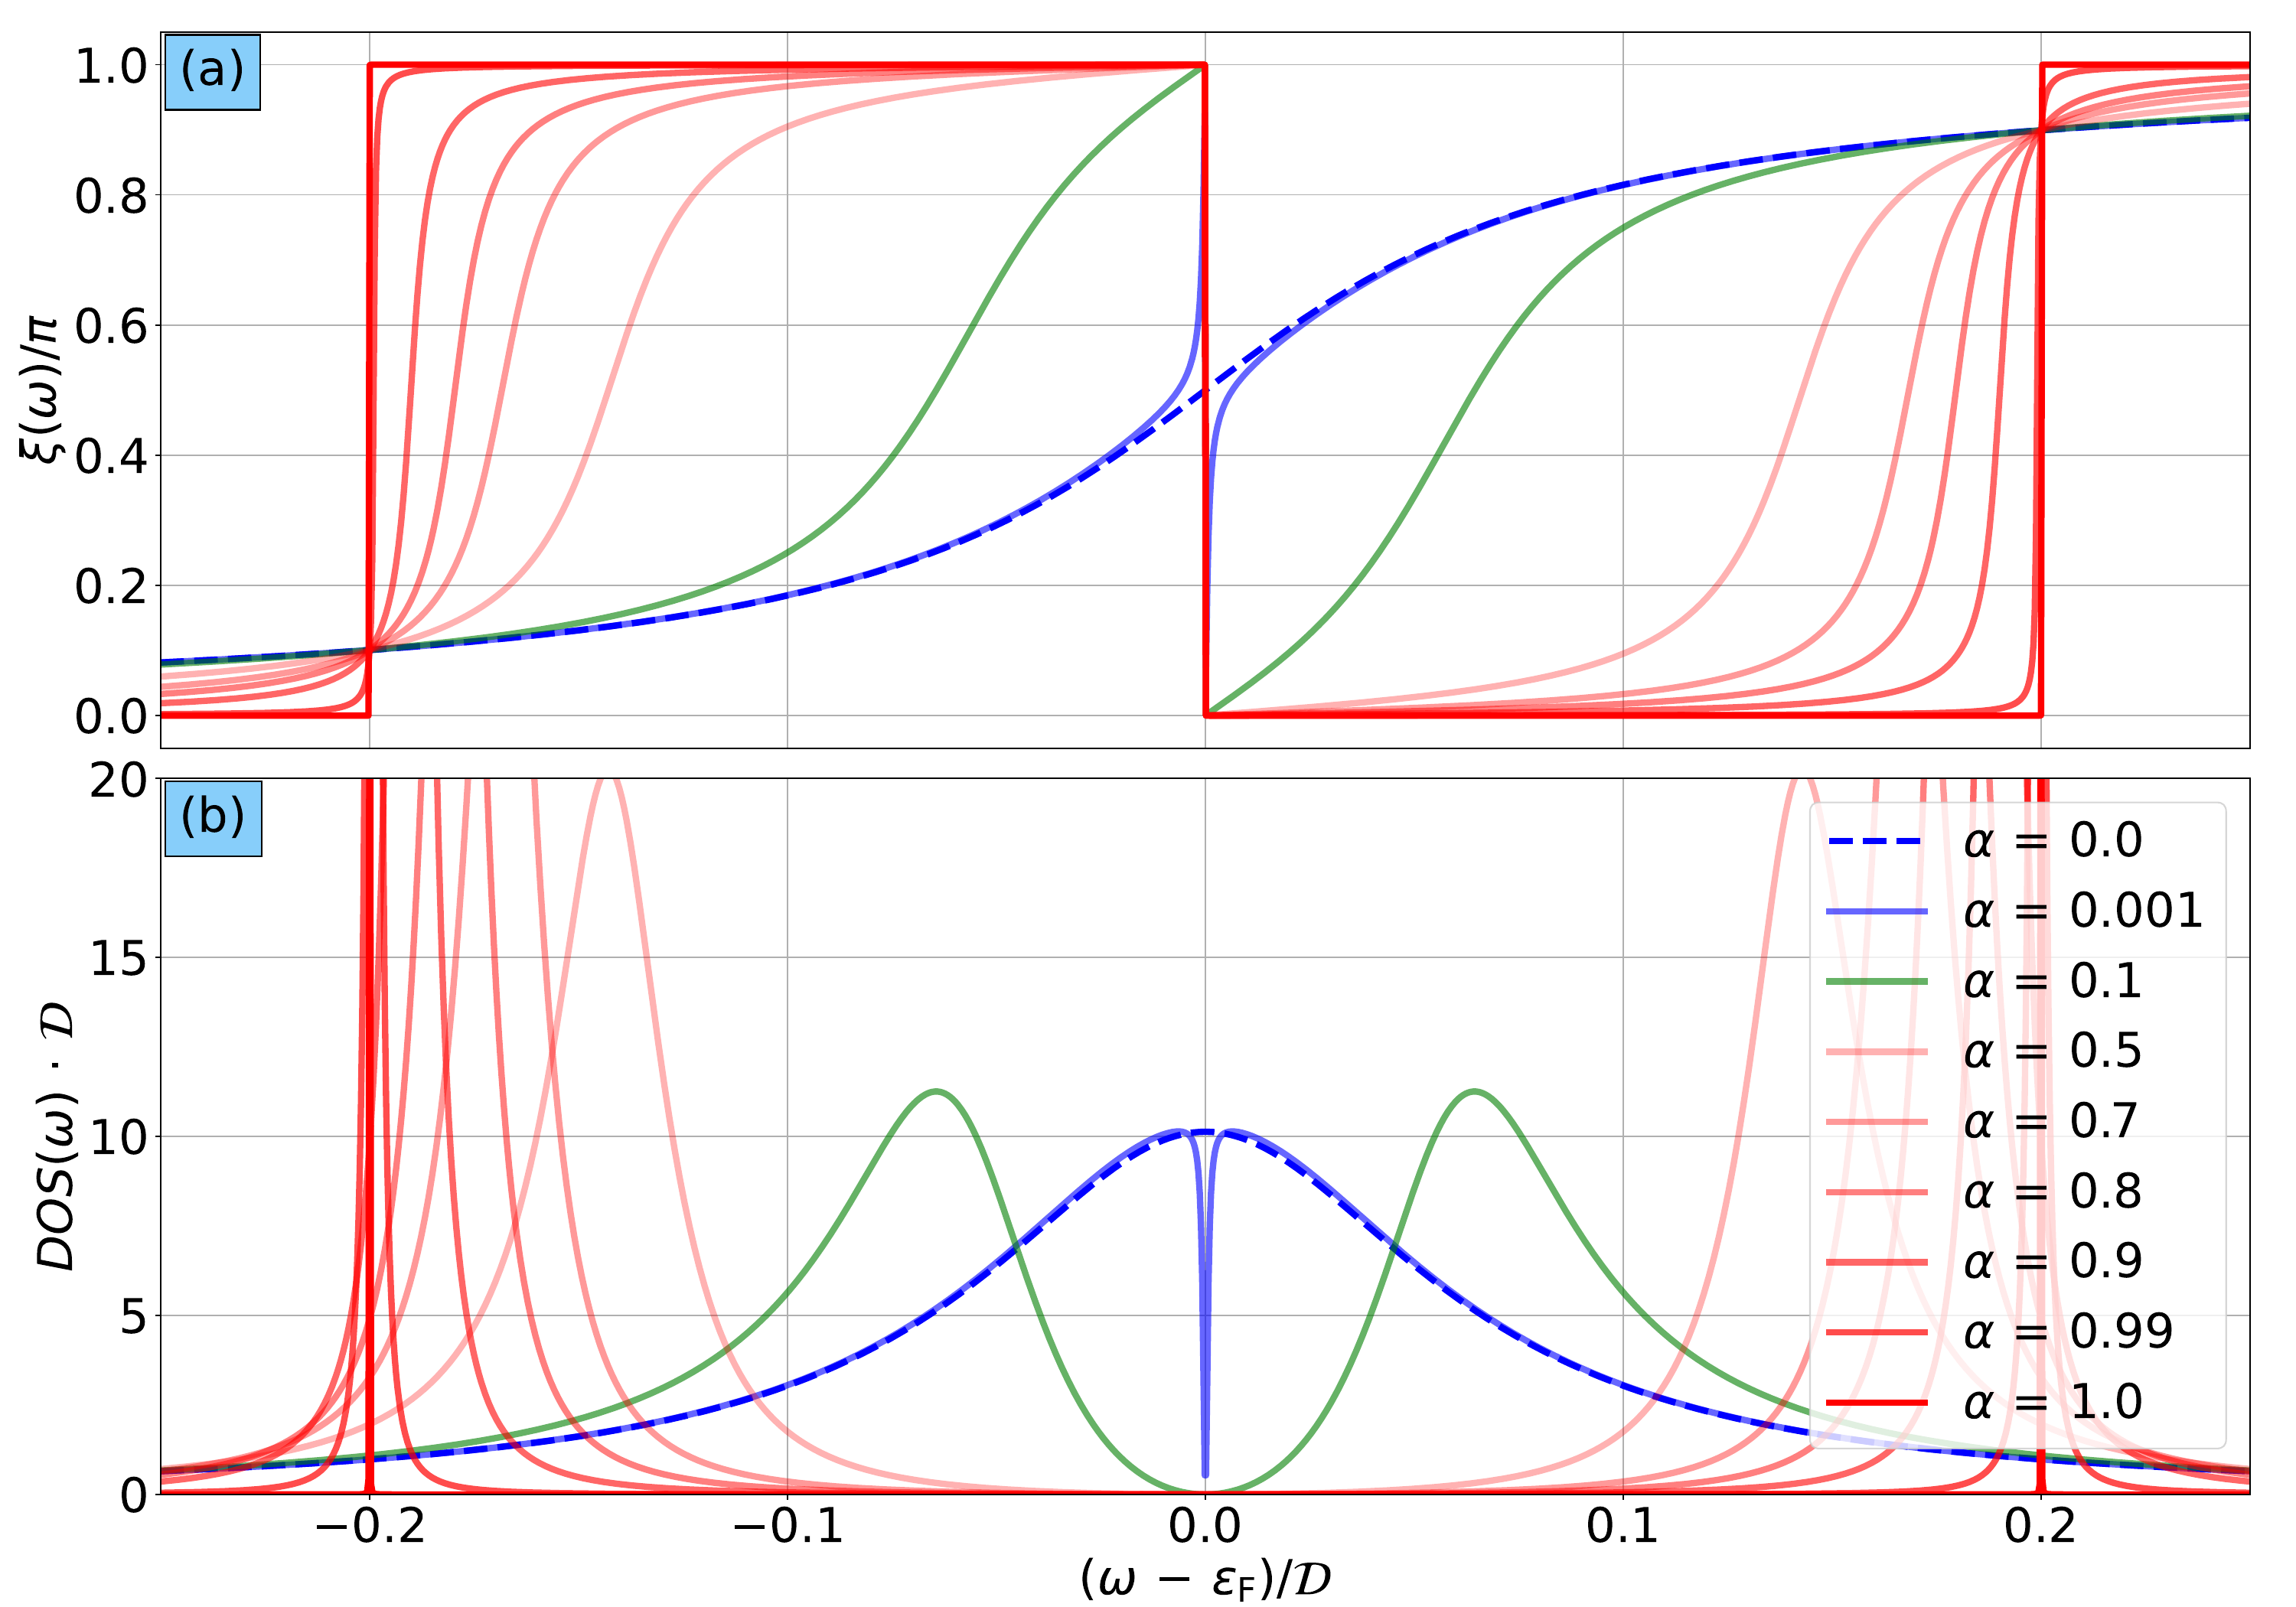}
    \caption{\justifying Scattering phase shift (a) and impurity density of states (b) for the non-interacting ($U=0.0\,\mathcal{D}$) single-site Anderson impurity model at $V=0.2\,\mathcal{D}$ and different values of the weight $\alpha$ from the main text.}
    \label{fig:scattering_phase_shift_and_impurity_DOS}
\end{figure*}\\
\noindent For a value of $\xi(\omega)\,=\,\frac{\pi}{2}$ the system consisting of the impurity level and the electron bath is in resonance, leading to a peak in the impurity density of states. At $\alpha\,=\,0$ this yields the Kondo peak at the Fermi level. By increasing $\alpha$, the resonance splits symmetrically around the Fermi level. At $\omega\,=\,\varepsilon_{F}$ the phase shift displays a jump by $\pi$.
\newpage
\subsection{Generalized charge susceptibility}
\noindent In the main text we analyzed the contribution of the bubble and vertex corrections to the local spin susceptibility depending on the weight of the central $\delta$-peak controlled by the parameter $\alpha$. Here, we are interested in the behavior of the two particle generalized charge susceptibility $\chi^{\text{charge}}_{\nu\nu'\omega}$ with respect to the chosen value of $\alpha$. This quantity including the Matsubara frequencies $\nu$ and $\nu'$ considers also two particle interactions and yields the impurity charge susceptibility of the main text after summation over the frequencies. The general static form ($\omega\,=\,0$) of this quantity reads:
\begin{equation}
    \chi^{\text{charge}}_{\nu\nu'}\,=\,\chi^{\uparrow\uparrow}_{\nu\nu'}\,+\,\chi^{\uparrow\downarrow}_{\nu\nu'}
\end{equation}
with
\begin{equation}
    \begin{split}
        \chi^{\sigma\sigma'}_{\nu\nu'}\,&=\,\int^{\beta}_0\,\text{d}\tau_1\,\text{d}\tau_2\,\text{d}\tau_3\,e^{-i\,\nu\,\tau_1}\,e^{i\,\nu\,\tau_2}\,e^{-i\,\nu'\,\tau_3}\,\times\\
        &\,\,\,\,\,\,\,\,\,\times\,\big[\big<T_\tau\,\hat{f}^\dagger_{\sigma}(\tau_1)\,\hat{f}_{\sigma}(\tau_2)\,\hat{f}^\dagger_{\sigma'}(\tau_3)\,\hat{f}_{\sigma'}(0)\big>\,-\big<T_\tau\hat{f}^\dagger_{\sigma}(\tau_1)\hat{f}_{\sigma}(\tau_2)\big>\big<T_\tau\hat{f}^\dagger_{\sigma'}(\tau_3)\hat{f}_{\sigma'}(0)\big>\big]\,.
    \end{split}
\end{equation}

\begin{figure*}[ht!]
    \centering
    \includegraphics[width=0.99\textwidth]{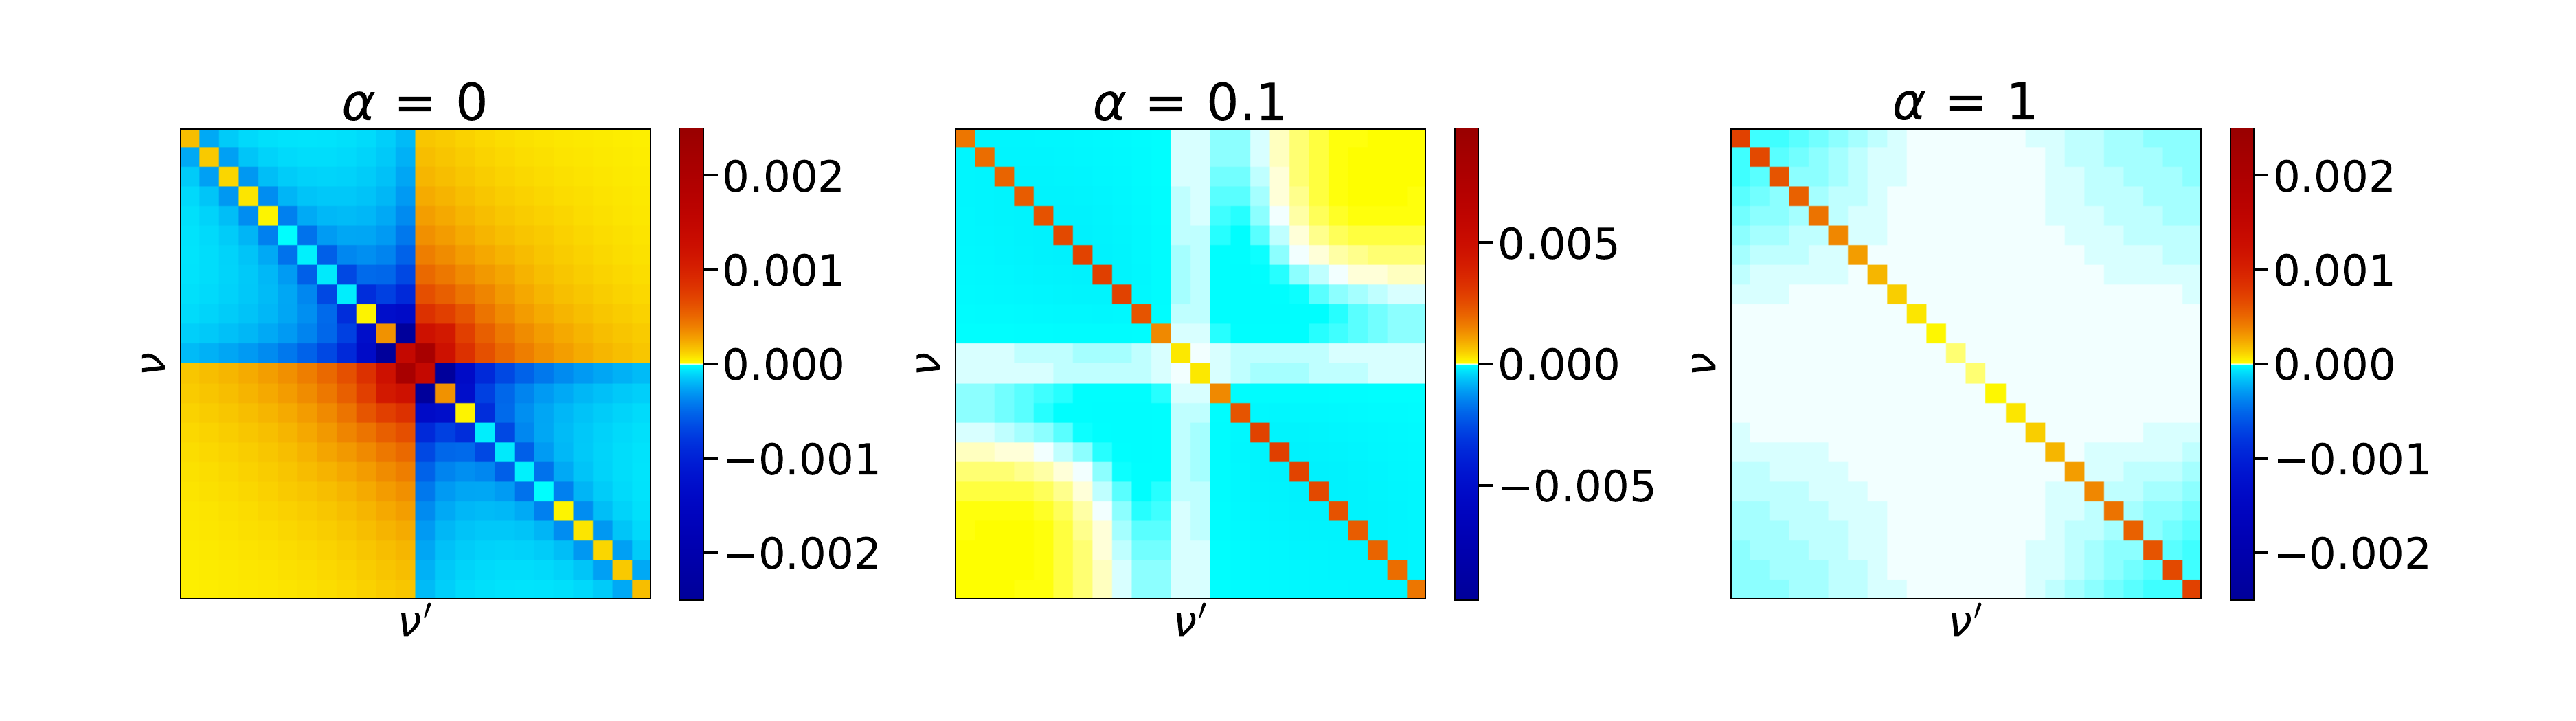}
    \caption{\justifying Matrices of the generalized static charge susceptibility at $T\,\approx\,0.0017\,\mathcal{D}$ for $\alpha\,=\,0$ (left), $\alpha\,=\,0.1$ (center) and $\alpha\,=\,1$ (right). The onion-like structure of the continuous hybridization ($\alpha\,=\,0$) vanishes due to the weight of the $\delta$-peak in the hybridization function leading to a minimum at small Matsubara frequencies in the center of the matrix.}
    \label{fig:colorplots_general_chi}
\end{figure*}

\noindent The matrix of the generalized charge susceptibility $\chi^{\text{charge}}_{\nu\nu'}$ is plotted in FIG.\,\ref{fig:colorplots_general_chi} for different values of $\alpha$. For $\alpha\,=\,0$ we are able to reproduce an onion-like structure, discussed in \cite{PhysRevLett.126.056403}, with a perturbative region at larger frequencies, a local moment regime at intermediate frequencies and a region at small frequencies, where the local moment is screened. The screening leads to a relaxation of the generalized charge susceptibility. Increasing $\alpha$ destroys the local moment together with the screening features, yielding two regimes: (i) a perturbative region at large frequencies and (ii) a region at smaller frequencies, where the diagonal is suppressed. Off-diagonal entries also decrease with $\alpha$. The suppression of $\chi^{\text{charge}}_{\nu,\,\nu'}$ depends on the weight of the hybridization function around the Fermi level.\\

\newpage
\subsection{Derivation of the RG flow equations}
\vspace{-2pt}
\noindent Our RG calculations are based on the Kondo Hamiltonian Eq.~(\ref{eq:Kondo_Hamiltonian}) of the main text. Here, we introduced the Abrikosov pseudospin ${\mathbf{S}\,=\,\hat{f}^\dagger_{\sigma}\,\frac{\boldsymbol{\sigma}_{\sigma,\sigma'}}{2}\,\hat{f}_{\sigma'}}$ with the constraint $\sum_\sigma\,\hat{f}^\dagger_{\sigma}\,\hat{f}_\sigma\,=\,1$. 
The action can be written as
\begin{equation}
\begin{split}
    \mathcal{S}\,=\,\int^{\beta}_{0}\,\text{d}\tau\,\Bigg[&\bar{f}_\sigma\,\partial_\tau\,f_\sigma\,+\,\int_{-\Lambda_0}^{\Lambda_0}\,\text{d}k\,\bar{c}_\sigma(k,\,\tau)\,\left(\partial_\tau\,-\,k\right)\,c_\sigma(k,\,\tau)\,-\,J\,\left(\bar{f}_\sigma\,\frac{\boldsymbol{\sigma}_{\sigma,\sigma'}}{2}\,f_{\sigma'}\right)\,\cdot\,\left(\bar{c}_\sigma(0)\,\frac{\boldsymbol{\tau}_{\sigma,\sigma'}}{2}\,c_{\sigma'}(0)\right)\\
    &+\,\bar{d}_{\sigma}\,\partial_\tau\,d_{\sigma}\,-\,K\,\left(\bar{f}_{\sigma}\,\frac{\boldsymbol{\sigma}_{\sigma,\sigma'}}{2}\,f_{\sigma'}\right)\,\cdot\,\left(\bar{d}_{\sigma}\,\frac{\boldsymbol{\tau}_{\sigma,\sigma'}}{2}\,d_{\sigma'}\right)\\
    &-\,M\,\left(\bar{f}_{\sigma}\,\frac{\boldsymbol{\sigma}_{\sigma,\sigma'}}{2}\,f_{\sigma'}\right)\,\cdot\,\left(\bar{c}_\sigma(0)\,\frac{\boldsymbol{\tau}_{\sigma,\sigma'}}{2}\,d_{\sigma'}\,+\,\bar{d}_\sigma\,\frac{\boldsymbol{\tau}_{\sigma,\sigma'}}{2}\,c_{\sigma'}(0)\right)\Bigg]\,,
\end{split}
\end{equation}
subject to the constraint on the $f$-fermions. Note that we introduced an energy cutoff $\Lambda$ consistent with the main text, and the fermions are represented by Grassmann variables. The Kondo couplings are related to that of the Anderson model in Eq.~\eqref{eq:general_AIM_Hamiltonian} of the main text as $J=(1-\alpha) J_0$, $K=\alpha J_0$, $M=\sqrt{\alpha(1-\alpha)} J_0$ with $J_0 = 2|V|^2 (1/|\epsilon_{f}| + 1/|\epsilon_{f}+U|)$, and we recall that $\alpha$ denotes the weight fraction of the peaked contribution of the Anderson-model hybridization function.
The scaling dimensions of the three coupling constants can be read off as
\begin{align}
    \text{dim}[J]\,=\,0\,,\,\,\,\,\,\,\,\,\,\,\text{dim}[K]\,=\,-1\,,\,\,\,\,\,\,\,\,\,\,
    \text{dim}[M]\,=\,-\frac{1}{2}\,.
\end{align}
The perturbative RG flow equations for the dimensionless running couplings $j$, $k$ and $m$ are given in Eq.~\eqref{eq:flow_equations} in the main text. Their linear terms are determined by the scaling dimension of the couplings; further terms describe contributions obtained by integrating out high-energy bath degrees of freedom. In our problem there are no $d$-fermions to be integrated out. The Kondo-only beta function arising for the $j$ coupling is known from previous RG calculations \cite{PhysRevB.70.214427}; perturbative renormalizations for $k$ and $m$ arise due to the presence of the mixed $m$ coupling. \\\\
\noindent In RG the running cutoff $\Lambda$ can directly be identified with temperature. We now analyze the temperature dependence of the couplings $j$, $k$ and $m$. Given that $k$ grows faster upon cooling than the other couplings, an initially small $k$ can become the dominant coupling at low temperature. By solving the flow equations, we qualitatively identify four different regions depending on the parameter $\alpha$ as follows:

\begin{itemize}
\item
(i) For $\alpha>1/2$ the flat-band coupling $k$ dominates for all $T$, implying that conventional Kondo screening is absent.

\item
(ii,iii) For intermediate $\alpha$ we see that $j$ dominates at elevated $T$, but $k$ wins at low $T$. Therefore, conventional Kondo screening is present, but cut off by the flat-band effects at a small energy or temperature scale, leading e.g. to a splitting of the Kondo peak. Regimes (ii) and (iii) are distinguished by whether this crossover happens above or below $T_K$, the Kondo temperature associated with the regular part of the hybridization.

\item
(iv) For very small $\alpha$ conventional Kondo screening dominates down to lowest $T$, i.e., $j$ flows to strong coupling before $k$ and $m$ become sizable. If we ignore the cross-coupling terms in the RG equations, we can estimate regime (iv) as $\alpha \ll T_K/\Lambda_0$.

\end{itemize}

A numerical solution of the RG equations is illustrated in Fig.~\ref{fig:Sketch_RG_alpha_temperature_regimes} of the main text.

\newpage
\subsection{Calculations off half-filling}
\,\\
For calculations away from half-filling, we perform QMC calculations with the software package w2dynamics \cite{Wallerberger_2019}. As first step we solve the impurity model at different temperatures for several values of the chemical potential $\mu$ where the desired occupation $n$ is included. Next, we apply an optimization algorithm on the chemical potential minimizing the difference of the occupation to the desired value. We use the chemical potential with appropriate accuracy and compute the local spin susceptibility $\chi^{\text{spin}}_{zz}$ with larger statistics. Thus, by fixing $\alpha$, the interaction $U\,=\,0.575\,\mathcal{D}$ and the occupation on the impurity site, we investigate $\chi^{\text{spin}}_{zz}$ away from half-filling as a function of the temperature $T/\mathcal{D}$. FIG.\,\ref{fig:local_spin_susceptibility_oohf_DOS} shows the behavior for $\alpha\,=\,0$ (a), $\alpha\,=\,0.5$ (b) and $\alpha\,=\,1$ (c) and assumes an occupation of $n\,=\,1.0$, $n\,=\,1.1$ and $n\,=\,1.25$ each. Starting with $\alpha\,=\,0$ the curve of $\chi^{\text{spin}}_{zz}$ approaches the plateau for small temperatures at lower values of $\chi^{\text{spin}}_{zz}$ with larger impurity occupations. This confirms that the screening effect of the bath electrons is supported by the raising probability of double occupation on the impurity site with the increasing occupation. Thus, the spin-$z$ expectation value is lowered, with a direct impact on the local spin susceptibility. For $\alpha\,=\,0.5$ (FIG.\,\ref{fig:local_spin_susceptibility_oohf_DOS} (b)) and $\alpha\,=\,1$ (FIG.\,\ref{fig:local_spin_susceptibility_oohf_DOS} (c)) the effect on $\chi^{\text{spin}}_{zz}$ is less prominent. Here, the curves exhibit a plateau at small temperatures coming from the favored singlet ground state of a Kondo dimer having a larger influence with increasing $\alpha$. This plateau decreases slightly with the impurity occupation. At intermediate temperatures the curves for different fillings and $\alpha\,\neq\,0$ show a maximum independent on the corresponding occupation on the impurity. However, the position of the maxima dependents on $\alpha$. Increasing it, slightly shifts the maximum to larger temperatures.  

\begin{figure*}
    \centering
    \includegraphics[width=0.99\textwidth]{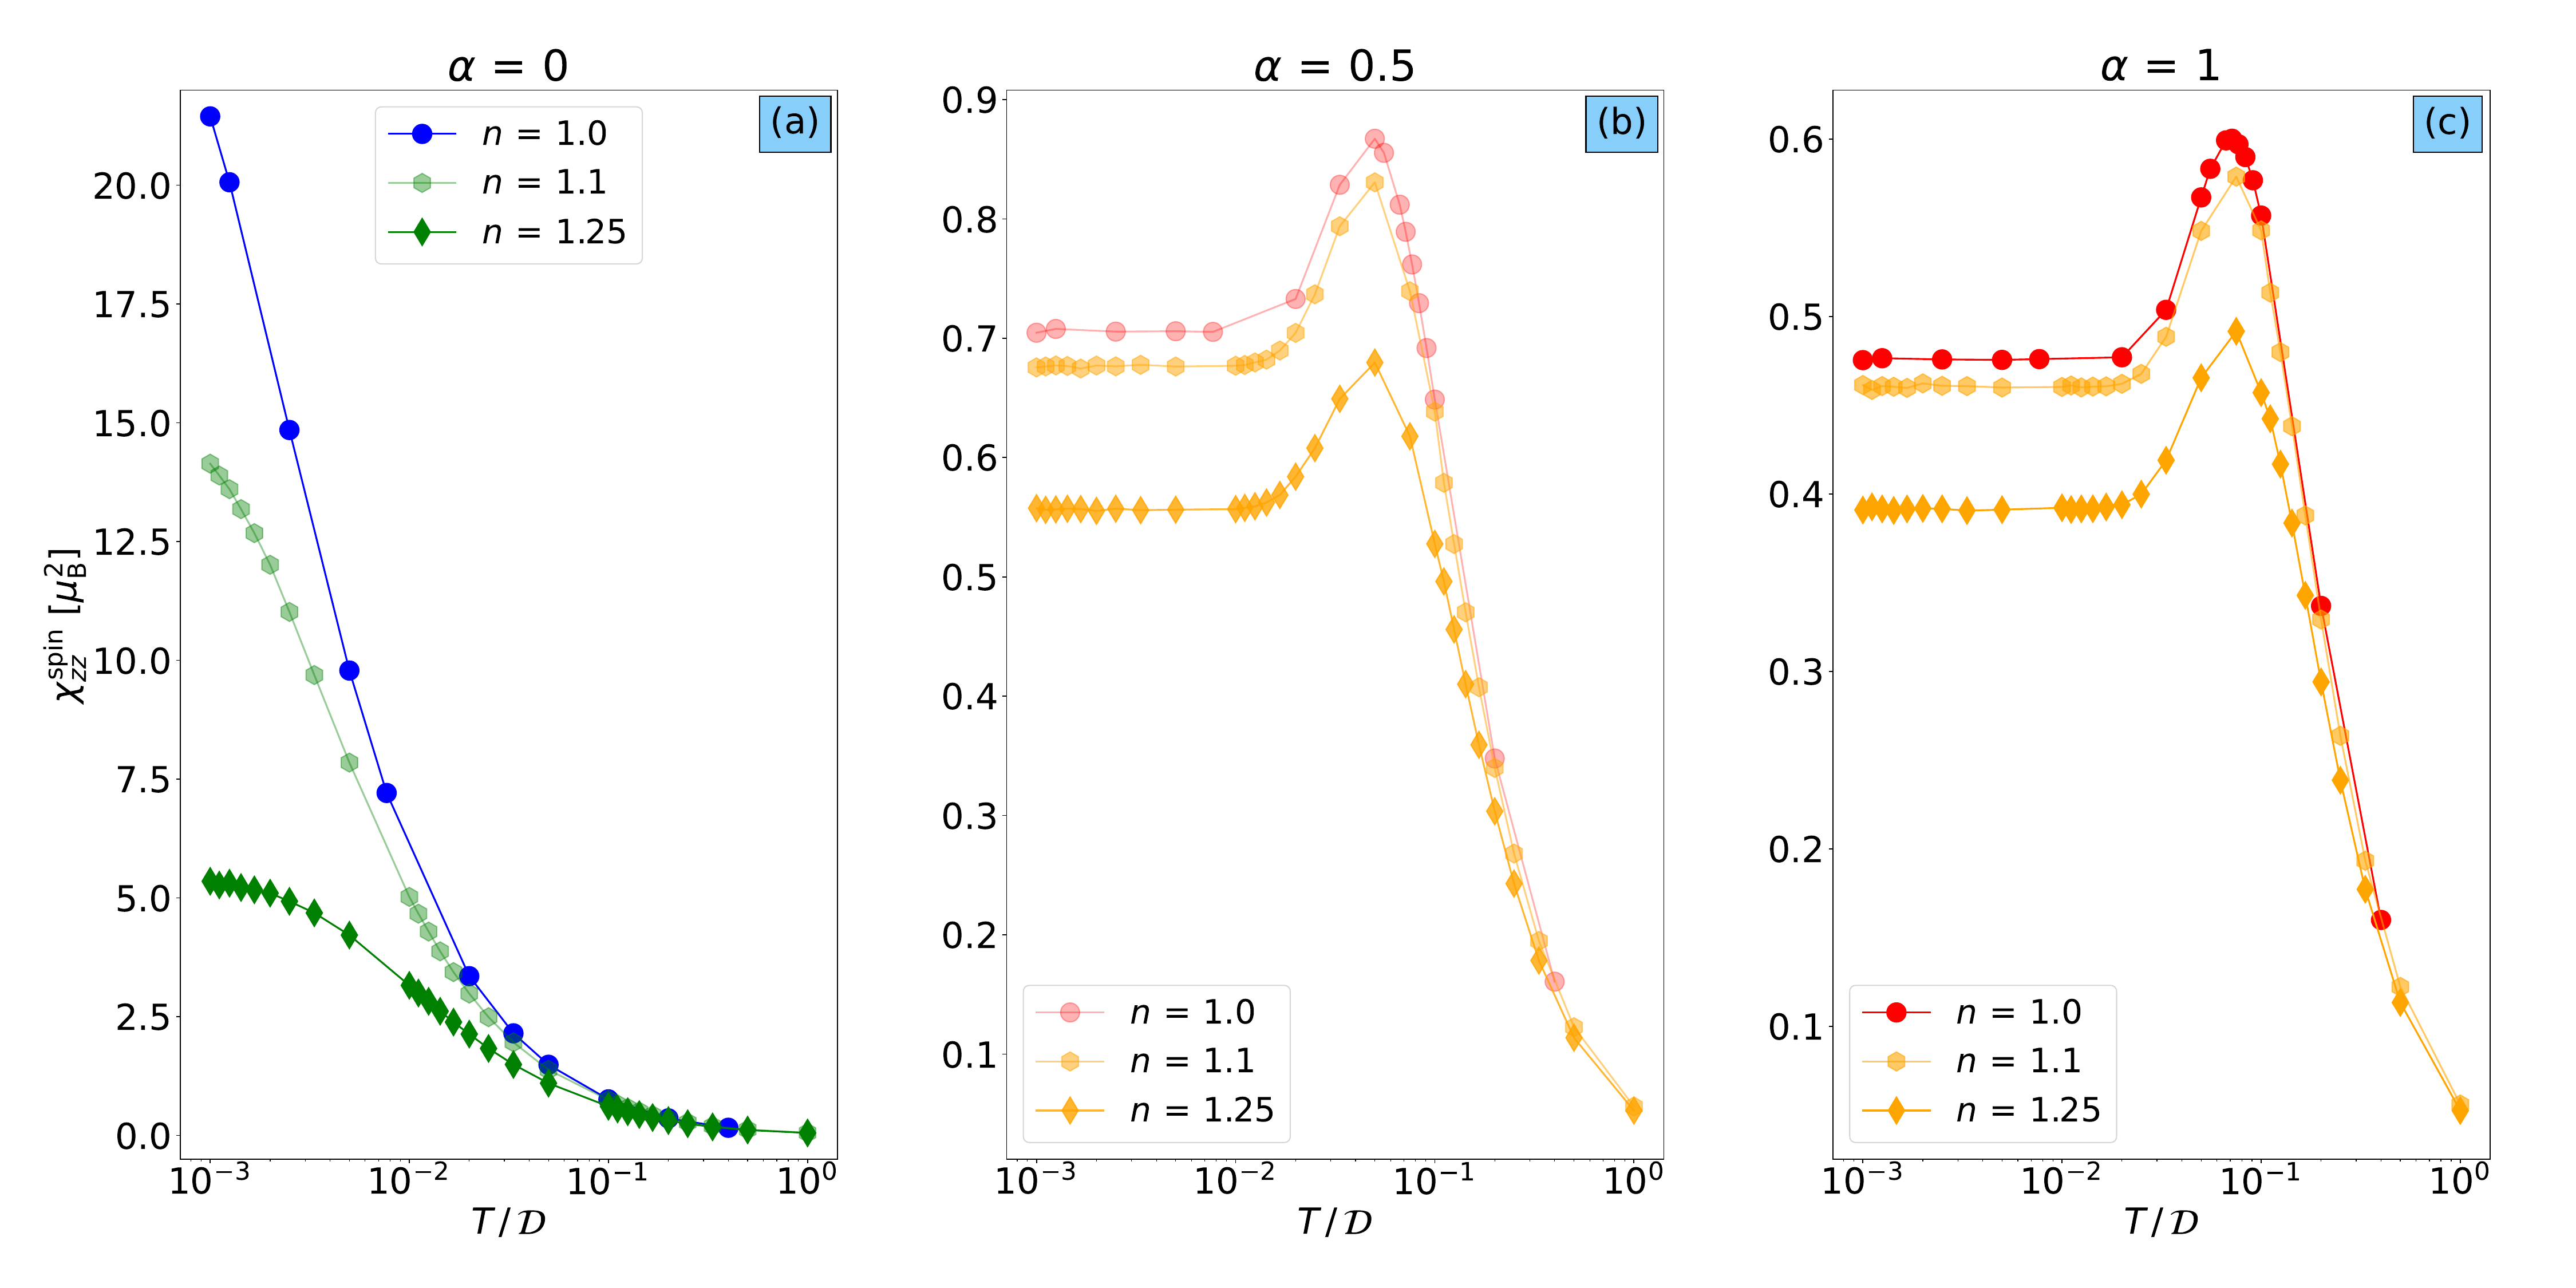}
    \caption{\justifying Local static spin susceptibility $\chi^{\text{spin}}_{zz}$ for several values of $\alpha$ and impurity occupations $n$ at $U\,=\,0.575\,\mathcal{D}$. The weight of the central $\delta$-peak increases from (a) to (c) with $\alpha\,=\,0$, $\alpha\,=\,0.5$ and $\alpha\,=\,1$. At small $\alpha$ the impact of the occupation on the impurity site has a large influence on the value of the plateau at small temperatures. Larger $\alpha$-values show qualitatively similar curves for different occupations. The positions of the maxima of the curves are independent on the respective impurity occupation but they highly depend on the weight $\alpha$.}
    \label{fig:local_spin_susceptibility_oohf_DOS}
\end{figure*}

\newpage
\subsection{Twisted bilayer graphene}
\newcommand{\DC}[1]{{\color{blue} \textbf{DC: #1}}}

\newcommand{\cmark}{\ding{51}}%
\newcommand{\xmark}{\ding{55}}%
\newcommand{\cre}[2]{{#1}^\dagger_{#2}}
\newcommand{\des}[2]{{#1}_{#2}}

\newcommand{\one}{\mathbb{1}}
\newcommand{\vk}{\vec{k}}
\newcommand{\vp}{\vec{p}}
\newcommand{\vK}{\vec{K}}
\newcommand{\vQ}{\vec{Q}}
\newcommand{\vq}{\vec{q}}
\newcommand{\vG}{\vec{G}}

\begin{figure}
    \centering
    \includegraphics[width=1.00\textwidth]{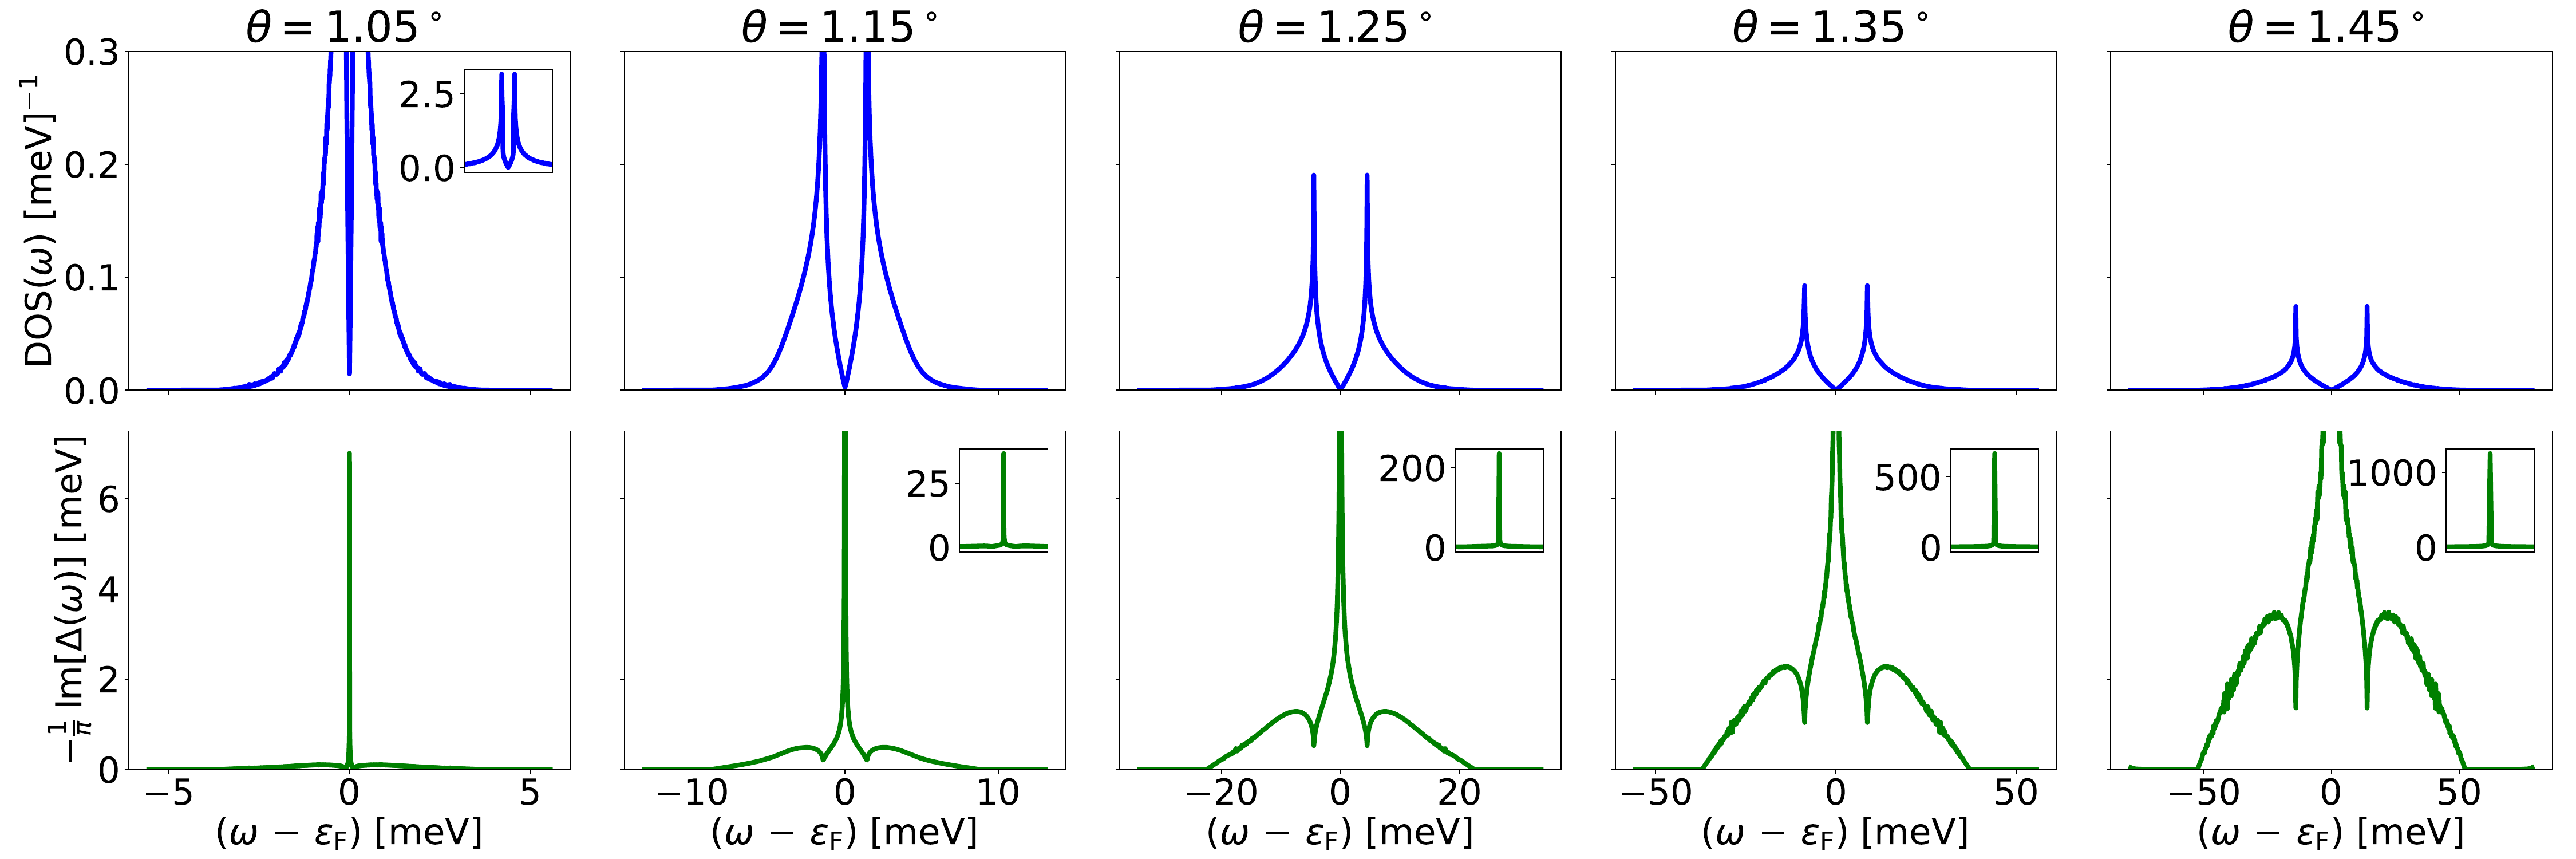}
    \caption{\justifying Impurity DOS$(\omega)$ and $-\frac{1}{\pi}\,\text{Im}[\Delta(\omega)]$ for twist angles of $\theta\,=\,1.05^{\circ}$, $\theta\,=\,1.15^{\circ}$, $\theta\,=\,1.25^{\circ}$, $\theta\,=\,1.35^{\circ}$ and $\theta\,=\,1.45^{\circ}$ (left to right) of twisted bilayer graphene for the THF model. The model always exhibits a 2 dimensional linear crossing at the $K$ point. In the hybridization function the zero weight of $-\frac{1}{\pi}\,\text{Im}\left[G_0(\omega)\right]$ at the Fermi level yields a peak superimposed on a smooth background, with a twist angle-dependent weight. The insets display the full $y$-range of the corresponding functions, while the frequency-range for the DOS is set at [$-1$m$eV$;$+1$m$eV$] and for $-\frac{1}{\pi}\,\text{Im}[\Delta(\omega)]$ at [$-5$m$eV$;$+5$m$eV$]). The values of the small imaginary part added to the real frequencies that we used are: $\eta\,=\,0.001$ for magic angle ($\theta\,=\,1.05^{\circ}$) and $\eta\,=\,0.01$ for other twist angles. For a better representation of the hybridization function, Fig.\,\ref{fig:sketch} of the main text has the value $\eta\,=\,0.1$.}
    \label{fig:DOS_hyb_func_magic_angle_1_40}
\end{figure}
\noindent To obtain the hybridization function of twisted bilayer graphene (TBG), we first require a localized Wannier orbital description of the system, analogous to the Anderson impurity model introduced in Sec.\,\ref{sec:system_Hamiltonian_hyb_func_expansion_low_freq}. For this purpose, we employ the topological heavy fermion (THF) model of TBG. In brief, the THF model is essentially a basis transformation of the low-energy TBG spectrum, in which its active bands emerge from the hybridization between localized, heavy, and strongly correlated $f$-fermions and topological, itinerant, and strongly dispersive $c$-electrons. In the THF basis, the single-particle Hamiltonian of the system is given by~\cite{PhysRevLett.129.047601,C_lug_ru_2023}:  
\begin{equation}
    \label{app:eqn:thf_non-int_ham}
    \hat{H}_{0}(\mathbf{k})\,=\,\sum_{\vert{\mathbf{k}}\vert{}<\Lambda_c}\,\sum_{a a' \eta s} H^{(c,\eta)}_{a a'}(\mathbf{k})\,c^{\dagger}_{\mathbf{k} a \eta s}c_{\mathbf{k} a' \eta s} + \frac{1}{\sqrt{N}} \sum_{\vert{\mathbf{k}}\vert{}<\Lambda_c}\,\sum_{\alpha a \eta s} \left[e^{i \mathbf{k}\cdot\mathbf{R} - \frac{\vert{\mathbf{k}}\vert{}^2 \lambda^2}{2}} H^{(fc,\eta)}_{\alpha a}(\mathbf{k}) f^{\dagger}_{\mathbf{R} \alpha \eta s} c_{\mathbf{k} \alpha \eta s} + \text{H.c.}\right]\,.
\end{equation}
\noindent In Eq.~\ref{app:eqn:thf_non-int_ham}, $\cre{c}{\mathbf{k} a \eta s}$ (for $1 \leq a \leq 4$) and $\cre{f}{\mathbf{R} \alpha \eta s}$ (for $\alpha = 1,2$) denote the creation operators for the $c$-electrons at momentum $\mathbf{k}$ and the $f$-electrons at lattice site $\mathbf{R}$, respectively. The Hamiltonian is diagonal in both the spin $s=\uparrow,\downarrow$ and valley $\eta=\pm$ indices. Because they are strongly dispersive, only the $c$-electrons with small momenta are relevant for the low-energy physics of the model; hence, a momentum cutoff $\Lambda_c$ is imposed for the $c$-electrons. The $f$-electrons are dispersionless but couple to the $c$-electrons through the second term in Eq.~\ref{app:eqn:thf_non-int_ham}. The hybridization function decays exponentially with momentum due to the finite spatial spread of the $f$ orbitals~\cite{PhysRevLett.129.047601,C_lug_ru_2023}, characterized by $\lambda$, the spread of the $f$-electron Wannier orbitals.

\noindent The corresponding matrix elements of the $c$ fermions have the form:
\begin{equation}
    H^{c,\eta}_{a a'}(\mathbf{k})\,=\,\begin{pmatrix}
        0_{2\times2} && v_* (\eta k_x \sigma_0 + i k_y \sigma_z) \\ v_* (\eta k_x \sigma_0 - i k_y \sigma_z) && M \sigma_x
    \end{pmatrix}
\end{equation}
and the hybridization between $f$- and $c$-fermions reads:
\begin{equation}
    H^{cf,\eta}_{a \alpha}(\mathbf{k})\,=\,\begin{pmatrix}
        \gamma \sigma_0 + v'_* (\eta k_x \sigma_x + k_y \sigma_y) \\ v''_* (\eta k_x \sigma_x - k_y \sigma_y)
    \end{pmatrix}\,.
\end{equation}
Here, all parameters are described within the context of the aforementioned papers. Near the magic angle, the $f$-electrons are dispersionless, but do acquire an intrinsic dispersion \emph{away} from the magic angle~\cite{C_lug_ru_2023}.\\\\
Remarkably, the THF mapping is applicable over a broad range of parameters, both at~\cite{PhysRevLett.129.047601} and away~\cite{C_lug_ru_2023} from the magic angle, and in the presence or absence of strain or lattice relaxation effects \cite{xv3m-vtlr}. To compute the hybridization function of the localized $f$-electron, one can, in principle, work directly within the THF model. However, away from the magic angle, a nearest-neighbor $f$-electron hopping must be included, and a sufficiently large cutoff $\Lambda_c$ is required to ensure that the low-energy dispersion of the active bands near the Dirac points is accurately reproduced.
\noindent
To circumvent these issues, we instead employ the continuum Bistritzer-MacDonald (BM) TBG Hamiltonian~\cite{doi:10.1073/pnas.1108174108}, which reads
\begin{equation}
	\label{app:eqn:plane_wave_ham}
	\hat{H}_{0} = \sum_{\mathbf{k}} \sum_{\eta, \alpha, \beta, s} \sum_{\mathbf{Q},\mathbf{Q}' \in \mathcal{Q}_{\pm}} \left[h^{\eta}_{\mathbf{Q},\mathbf{Q}'} \left( \mathbf{k} \right) \right]_{\alpha \beta} \cre{c}{\mathbf{k},\mathbf{Q},\eta,\alpha,s} \des{c}{\mathbf{k},\mathbf{Q}',\eta,\beta,s},
\end{equation}
where the definition of the plane-wave operators $\cre{c}{\mathbf{k},\mathbf{Q},\eta,\alpha,s}$, as well as the explicit form of the corresponding plane-wave Hamiltonian, is given in Ref.~\cite{PhysRevB.103.205413}. In the plane-wave basis, the wave function of the $f$-electrons is expressed as
\begin{equation}
	\label{app:eqn:f_fermions_mom_def}
	\cre{f}{\mathbf{k},\alpha,\eta,s} = \sum_{\mathbf{Q},\beta} v^{\eta}_{\mathbf{Q}\beta;\alpha} \left( \mathbf{k} \right) \cre{c}{\mathbf{k},\mathbf{Q},\beta,\eta,s},
\end{equation} 
with the coefficients $v^{\eta}_{\mathbf{Q}\beta;\alpha} \left( \mathbf{k} \right)$ obtained through a combined Wannierization and disentangling procedure. Using the plane-wave Hamiltonian and the wave function of the $f$-electrons, we can obtain the non-interacting $f$-electron Green's function. Specifically, we first compute the single-particle Green's function of the plane-wave Hamiltonian from Eq.\,\ref{app:eqn:plane_wave_ham},  
\begin{equation}
	\mathcal{G}^{\eta} \left( \omega, \mathbf{k} \right) = \left[ \left( \omega + i \eta \right) \one - h^{\eta} \left( \mathbf{k} \right) \right]^{-1},
\end{equation}
which can be straightforwardly projected onto the $f$-electron states
\begin{equation}
	\mathcal{G}^{f,\eta}_{\alpha \beta} \left( \omega, \mathbf{k} \right) = \sum_{\mathbf{Q},\mathbf{Q}' \in \mathcal{Q}_{\pm}} v^{*\eta}_{\mathbf{Q}\alpha';\alpha} \left( \mathbf{k} \right) \left[ \mathcal{G}^{\eta}_{\mathbf{Q},\mathbf{Q}'} \left( \omega, \mathbf{k} \right) \right]_{\alpha' \beta'} v^{\eta}_{\mathbf{Q}'\beta';\beta} \left( \mathbf{k} \right).
\end{equation}
The $ff$-block of the onsite non-interacting Green's function, which is orbital and valley diagonal, is subsequently obtained through Fourier transformation
\begin{equation}
	\label{app:eqn:greens_func_local}
	\frac{1}{N} \sum_{\mathbf{k}} \mathcal{G}^{f,\eta}_{\alpha \beta} \left( \omega, \mathbf{k} \right) = G_{0}\!\left( \omega \right)\!{\big\vert{}}_{ff}  \delta_{\alpha \beta}.
\end{equation} \\
In our numerical simulations we employed an $N = 1536 \times 1536$ $\mathbf{k}$-mesh and computed the non-interacting Green's function of the $f$-fermions at half-filling and particle-hole symmetry according to Eq.\,\ref{app:eqn:greens_func_local}. The hybridization function for the $f$-fermions is then defined as
\begin{equation}
    \Delta(\omega)\,=\,\omega\,+\,i\,\eta-\,\left[G_0(\omega){\big\vert{}}_{ff}\right]^{-1}\,.
\end{equation}
In Fig.\,\ref{fig:DOS_hyb_func_magic_angle_1_40} we summarized some plots of $-\frac{1}{\pi}\,\text{Im}\left[G_0(\omega)\right]$ and the hybridization function for the $f$-electrons choosing different twist angles. In fact, the bandstructure for the THF model always describes a two-dimensional linear crossing at the $K$ point leading to a peak in the hybridization function. Nonetheless, this peak can be resolved easier at larger twist angles, since the weight of the peak increases with the twist angle. 
\begin{figure}
    \centering
    \includegraphics[width=0.59\textwidth]{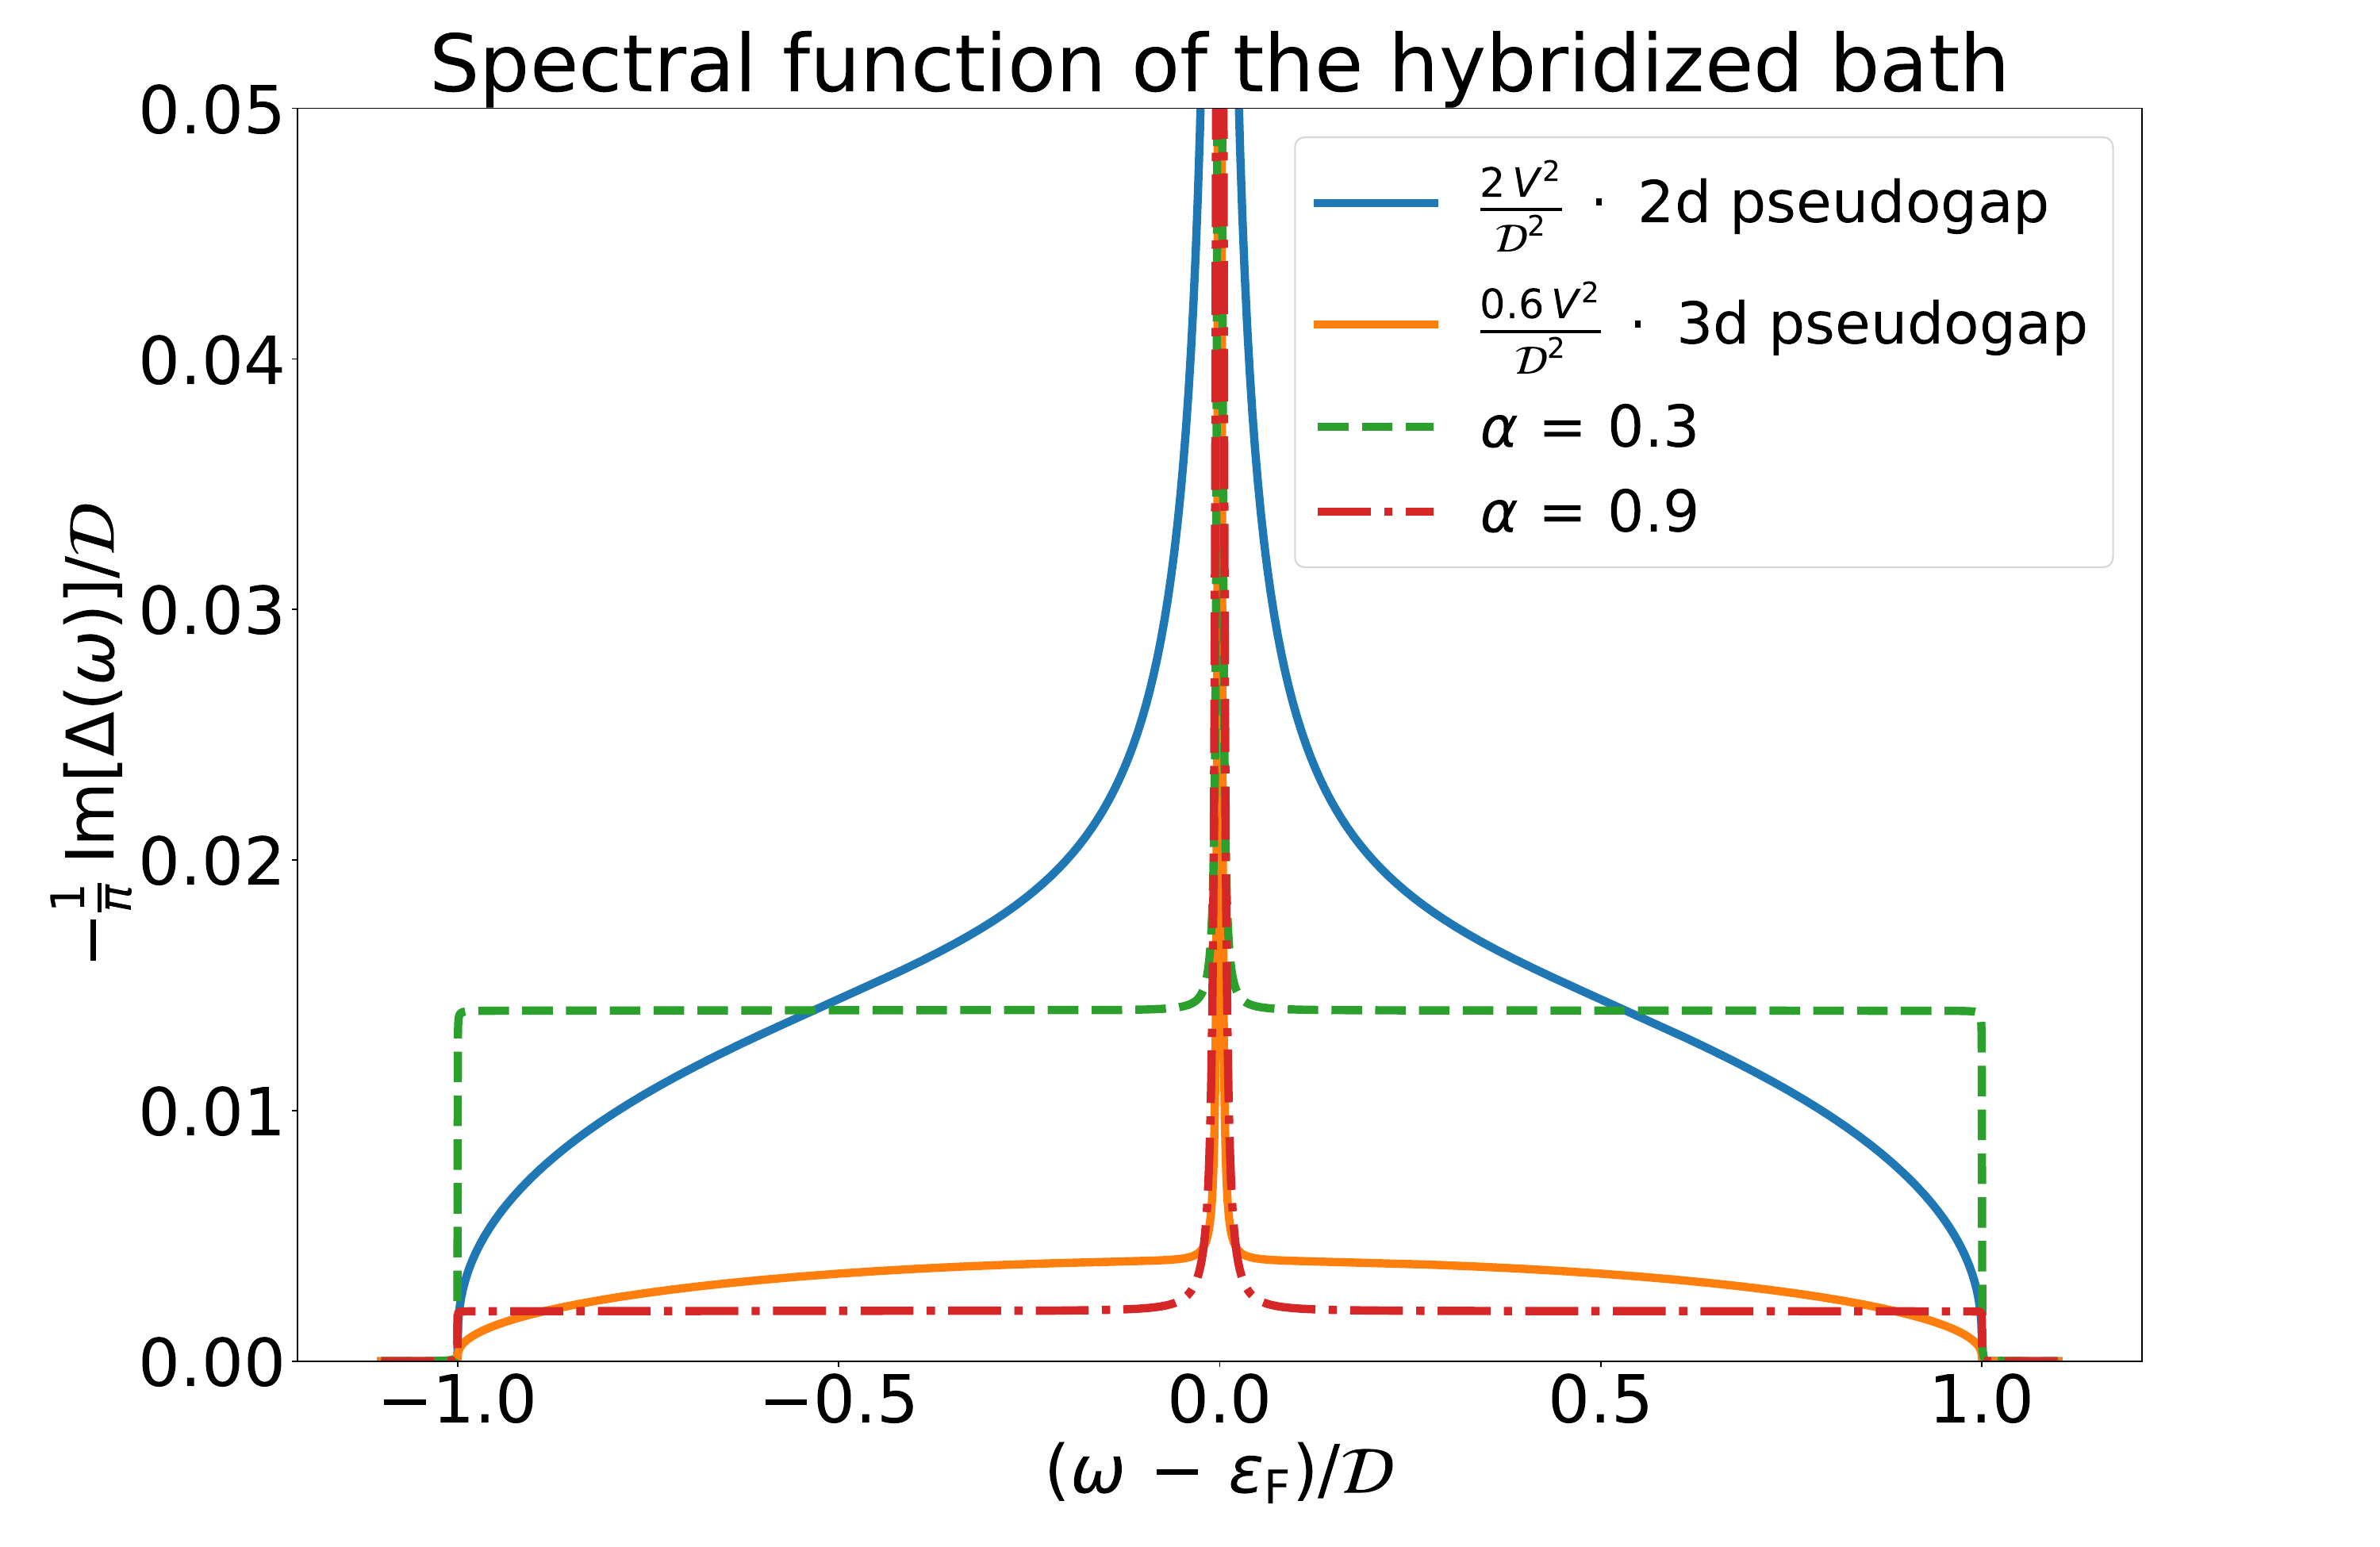}
    \caption{\justifying Imaginary part of hybridization functions $-\frac{1}{\pi}\,\text{Im}[\Delta(\omega)]/\mathcal{D}$ for 2d and 3d pseudogaps (blue and orange) together with the model of the main text combining a box-like hybridization with a central $\delta$-peak for two possible values of $\alpha$ ($\alpha\,=\,0.3$ in green and $\alpha\,=\,0.9$ in red) with a small imaginary part $\eta$ added to the frequency. The hybridization function for the 2d pseudogap is multiplied by the factor $\frac{2\,V^2}{\mathcal{D}^2}$ and for the 3d pseudogap by $\frac{0.6\,V^2}{\mathcal{D}^2}$, such that they are normalized to $V^2$. Parameters: $V\,=\,0.2\,\mathcal{D}$, $\eta\,=\,0.0001\,\mathcal{D}$.}
    \label{fig:Comparison_2d_3d_flat_plus_delta}
\end{figure}\\
\noindent In order to find the correct behavior of this peaked structure for the hybridization of the $f$-bands in TBG at low frequencies, we analyze a 2D pseudogap system with energy cutoff $\mathcal{D}$. Here, we have the linear dispersion $\epsilon_{\vert{\mathbf{k}}\vert{}}\,=\,\vert{\mathbf{k}}\vert{}$ in two dimensions and the density of states:
\begin{equation}
    -\frac{1}{\pi}\,\text{Im}\left[G_0(\epsilon)\right]\,\propto\,\int^{\infty}_{-\infty}\,\text{d}^2 \mathbf{k}\,\delta(\epsilon\,-\,\epsilon_{\vert{\mathbf{k}}\vert{}})\,\propto\,\int^{\infty}_{-\infty}\,\text{d} \vert{\mathbf{k}}\vert{}\,\vert{\mathbf{k}}\vert{}\,\delta(\epsilon\,-\,\vert{\mathbf{k}}\vert{})\,\propto\,\vert{\epsilon}\vert{}\,,
\end{equation}
with its normalized expression:
\begin{equation}
    -\frac{1}{\pi}\,\text{Im}\left[G_0(\epsilon)\right]\,=\,\frac{1}{\mathcal{D}^2}\,\vert{\epsilon}\vert{}\,.
\end{equation}
Following the procedure of Sec.\,\ref{sec:system_Hamiltonian_hyb_func_expansion_low_freq}, the non-interacting Green's function $G_0$ reads:
\begin{equation}
    G_0(\omega)\,=\,\frac{\left(\omega\,+\,i\,\eta\right)}{\mathcal{D}^2}\,\ln{\left(\frac{\left(\omega\,+\,i\,\eta\right)^2}{\left(\omega\,+\,i\,\eta\right)^2\,-\,\mathcal{D}^2}\right)}\,.
\end{equation}
By taking the limits $\omega\,\rightarrow{0}$ and $\eta\,\rightarrow{0}$ the logarithm becomes $\ln{\left(\frac{\left(\omega\,+\,i\,\eta\right)^2}{\left(\omega\,+\,i\,\eta\right)^2\,-\,\mathcal{D}^2}\right)}\,\approx\,x\,+\,i\,y\,-\,i\,z$, with $x\,=\,\ln{\left(\frac{\omega^2\,+\,\eta^2}{\mathcal{D}^2}\right)}$, $y\,=\,\arctan{\left(-\frac{2\,\omega\,\eta}{\eta^2\,-\,\omega^2}\right)}$ and $z\,=\,\pi\,\text{sig}(\omega)$, yielding:
\begin{equation}
    G_0(\omega)\,=\,G'_0\,+\,i\,G''_0\,\approx\,\frac{\left(\omega + i\eta \right)}{\mathcal{D}^2}\,\left(x\,+\,i\,y\,-\,i\,z\right).
\end{equation}
This leads to the imaginary part of the hybridization functions for $\omega\,\rightarrow{0}$ and $\eta\,\rightarrow{0}$:
\begin{equation}
    -\frac{1}{\pi}\,\text{Im}\left[\Delta(\omega)\right]\,=\,-\frac{1}{\pi}\,\left[\eta\,+\,\frac{G''_0}{G'^2_0\,+\,G''^2_0}\right]\,\approx\,\mathcal{D}^2\,\text{sig}(\omega)\,\frac{1}{\omega\,\left(4\,\ln{\left(\frac{\omega}{\mathcal{D}}\right)}^2\,+\,\pi^2\right)}\,.
\end{equation}
Fig.\,\ref{fig:Comparison_2d_3d_flat_plus_delta} compares the quantity $-\frac{1}{\pi}\,\text{Im}[\Delta(\omega)]/\mathcal{D}$ for a two- and a three-dimensional pseudogap and the toy model of the main text for $\alpha\,=\,0.3$ and $\alpha\,=\,0.9$. Here, in all cases the full non-interacting Green's function was taken to calculate the hybridization functions. For the 2d pseudogap the curve was multiplied by $\frac{2\,V^2}{\mathcal{D}^2}$ and for the 3d-pseudogap by $\frac{0.6\,V^2}{\mathcal{D}^2}$ to be normalized to $V^2$.

\bibliographystyle{apsrev4-2}
\bibliography{bibliography}

\end{document}
