# Supplementary material for: Fragility of local moments against hybridization with flat bands
Source: arXiv:2503.14326 source file (2026-08-11)
Supplement: Supplementary file 2 [file Analytic_results_spin_charge_sus.tex]

\subsection{Analytic results for the spin and charge responses of a Kondo dimer at half-filling}
\label{sec:Analytic_results_Kondo_dimer_spin_charge_sus}
\noindent To construct a Kondo dimer, we assume a general Anderson impurity model with a single hybridization level and one impurity site:
\begin{equation}
   \hat{H}\,=\,\sum_{\sigma}\,\epsilon_{d}\,\hat{d}^{\dagger}_{\sigma}\,\hat{d}_{\sigma}\,+\,\sum_{\sigma}\,\epsilon_{f}\,\hat{f}^{\dagger}_{\sigma}\,\hat{f}_{\sigma}\,+\,V\,\sum_{\sigma}\,\left(\hat{d}^{\dagger}_{\sigma}\,\hat{f}_{\sigma}\,+\,\hat{f}^{\dagger}_{\sigma}\,\hat{d}_{\sigma}\right)\,+\,U\,\hat{n}_{f\uparrow}\,\hat{n}_{f\downarrow}\,,
\label{eq:AIM_Hamiltonian}
\end{equation}
with $d$ denoting quantities on the bath level and $f$ describing the impurity level. At half-filling the energy of the two levels are set to $\epsilon_f\,=\,-\frac{U}{2}$ and $\epsilon_d\,=\,0$, such that the Hamiltonian can be rewritten in the form:
\begin{equation}
    \hat{H}\,=\,U\,\hat{n}_{f\uparrow}\,\hat{n}_{f\downarrow}\,-\,\frac{U}{2}\,\left(\hat{n}_{f\uparrow}\,+\,\hat{n}_{f\downarrow}\right)\,+\,V\,\sum_{\sigma}\,\left(\hat{d}^{\dagger}_{\sigma}\,\hat{f}_{\sigma}\,+\,\hat{f}^{\dagger}_{\sigma}\,\hat{d}_{\sigma}\right)\,.
\end{equation}
This system can be solved analytically for the eigenenergies, summarized in TABLE\,\ref{tab:Kondo_dimer_energy_levels} and plotted in Fig.\,\ref{fig:histogramm_energy_levels} for $U\,=\,0$ (blue) and $U\,=\,5.75$ (orange) at the hybridization $V\,=\,2$ with the corresponding degeneracies. The prefactors $N_{ii}$ describe normalization factors for the eigenstates. 
\begin{figure}
    \centering
    \includegraphics[width=0.59\textwidth]{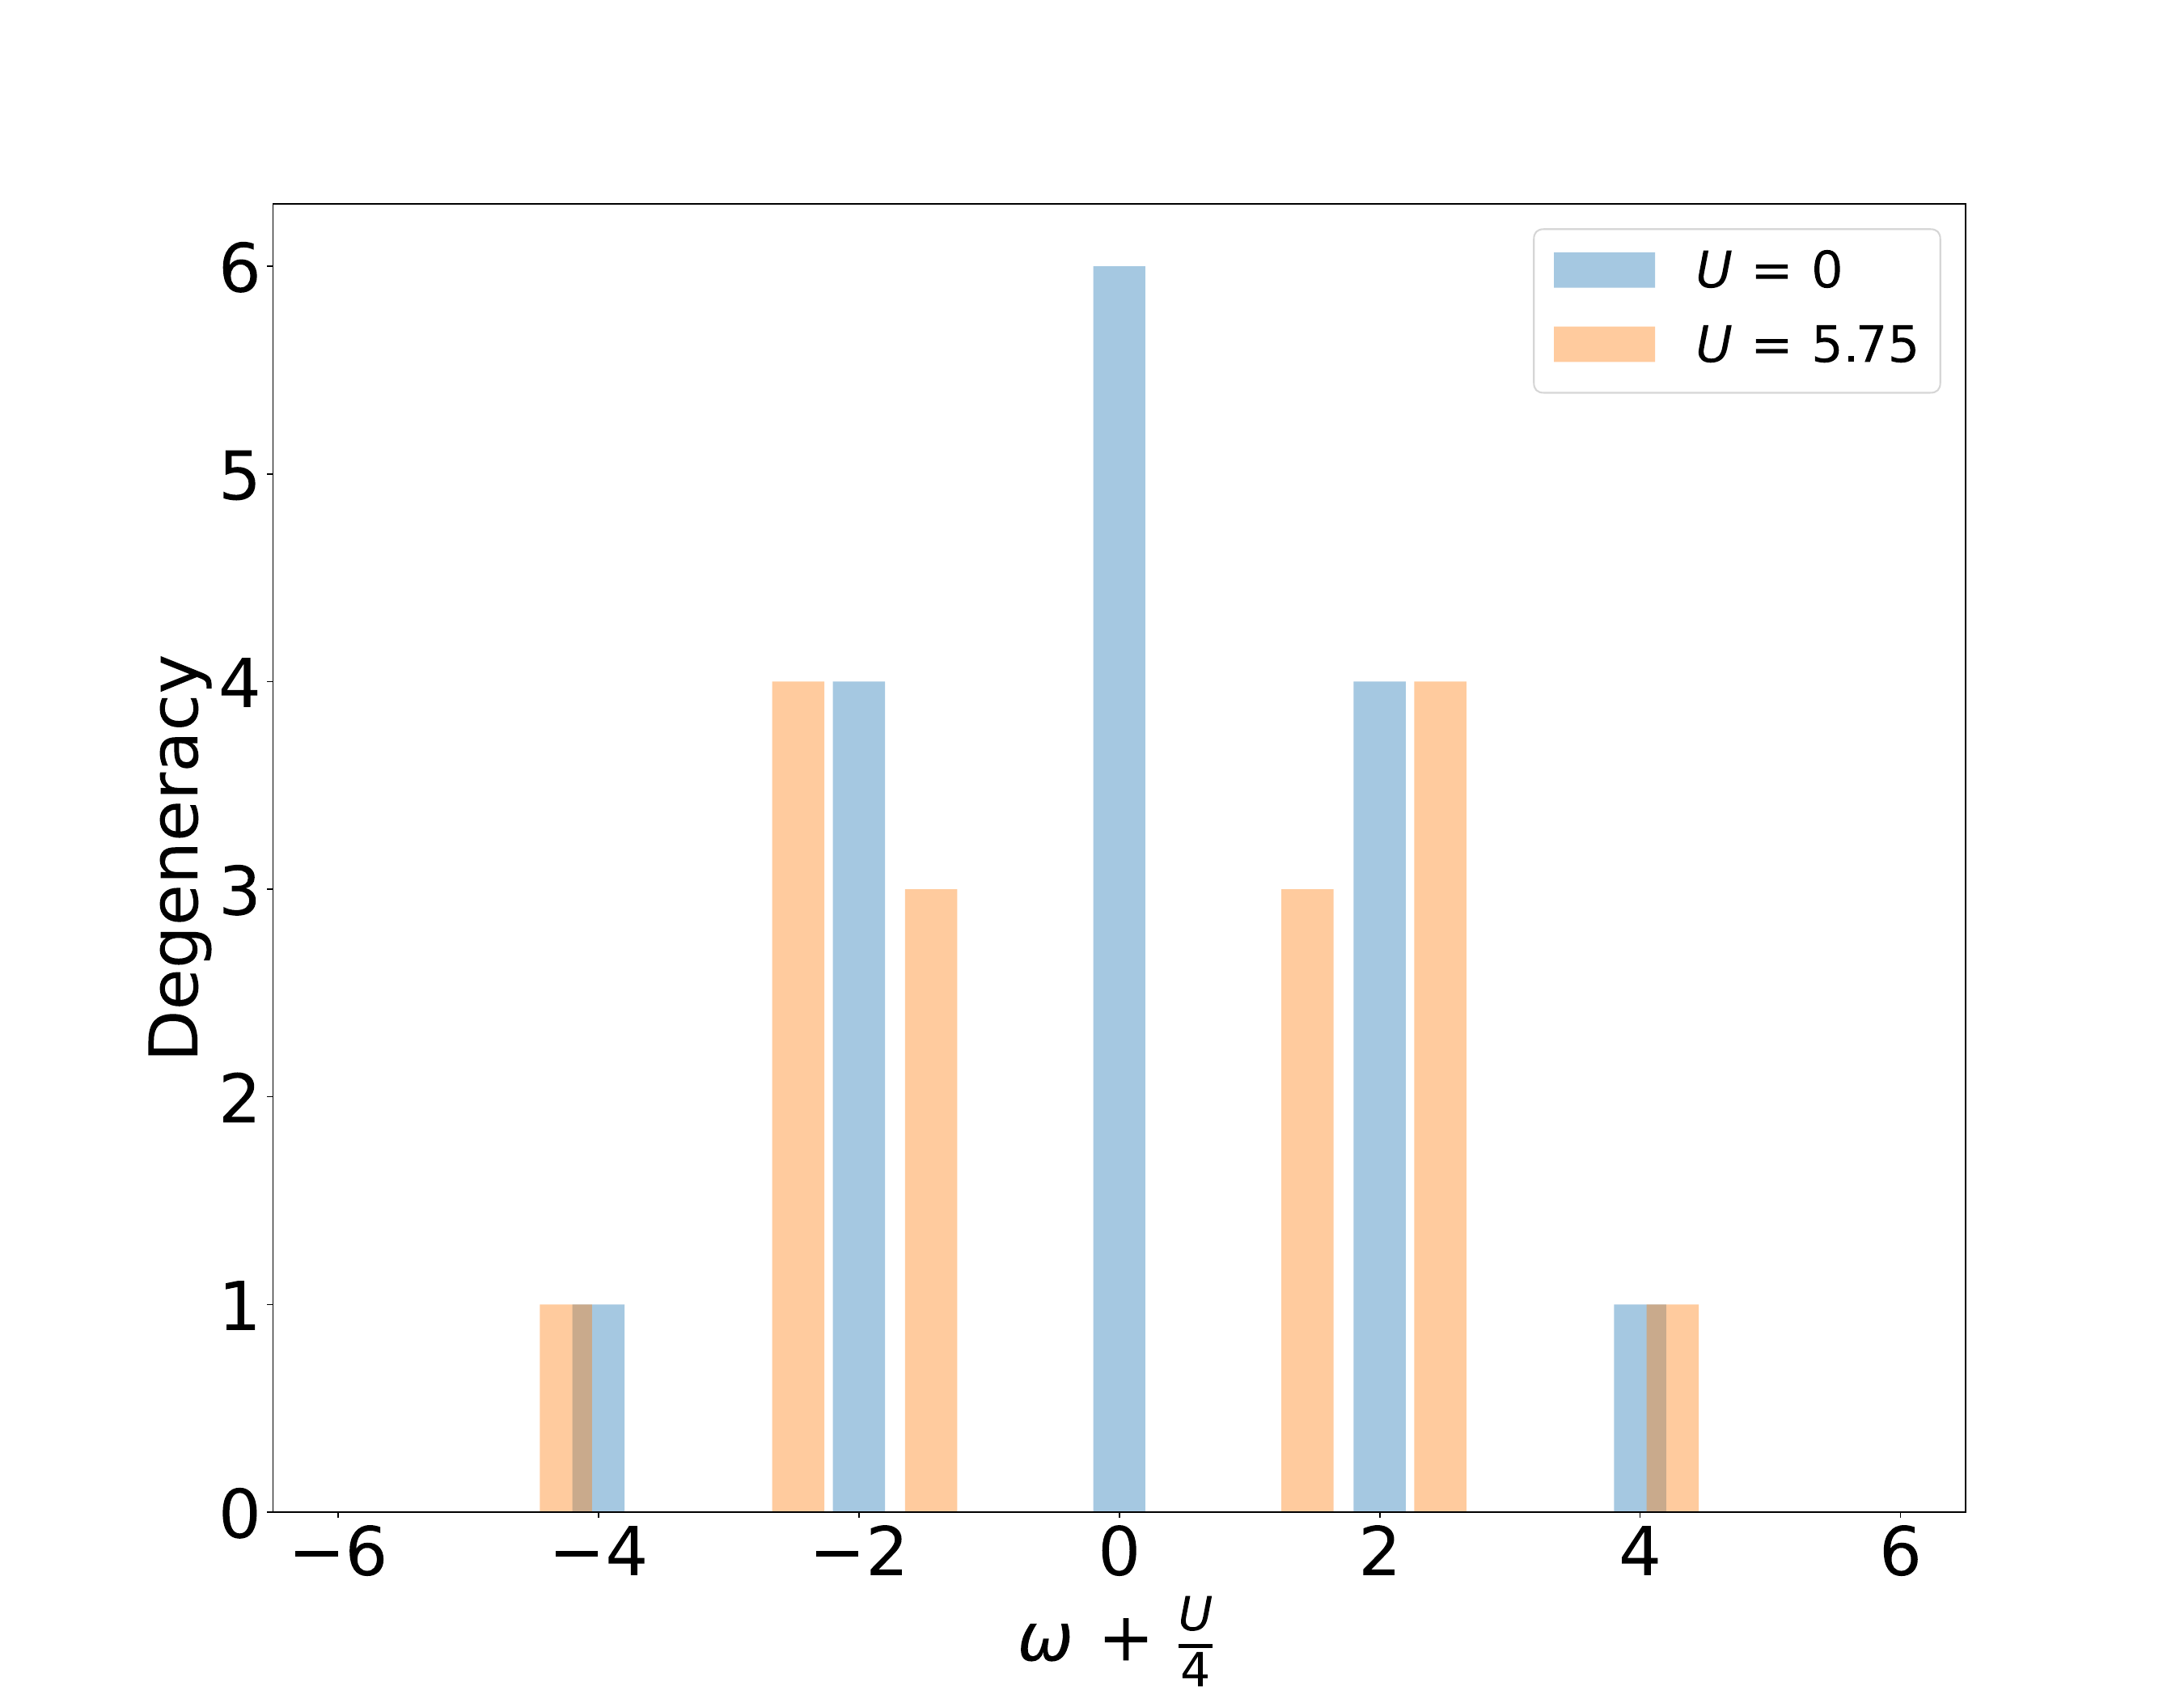}
    \caption{\justifying Energy levels of a Kondo dimer with one interacting site hybridized with a non-interacting site at half-filling with the interaction $U\,=\,0$ (blue) and $U\,=\,5.75$ (orange). Hopping between the sites is described by the hybridization $V\,=\,2$.}
    \label{fig:histogramm_energy_levels}
\end{figure}
With the eigenenergies we are able to establish the corresponding partition function:
\begin{equation}
    Z\,=\,\sum_n\,e^{-\beta\,\epsilon_n}\,=\,e^{-\beta\,\epsilon_0}\,+\,4\,e^{-\beta\,\epsilon_1}\,+\,3\,e^{-\beta\,\epsilon_2}\,+\,3\,e^{-\beta\,\epsilon_3}\,+\,4\,e^{-\beta\,\epsilon_4}\,+\,e^{-\beta\,\epsilon_5}\,,
\end{equation}
or by defining $\Delta_i\,=\,\epsilon_i\,-\,\epsilon_0$:
\begin{equation}
    Z\,=\,e^{-\beta\,\epsilon_0}\,\left(1\,+\,4\,e^{-\beta\,\Delta_1}\,+\,3\,e^{-\beta\,\Delta_2}\,+\,3\,e^{-\beta\,\Delta_3}\,+\,4\,e^{-\beta\,\Delta_4}\,+\,e^{-\beta\,\Delta_5}\right)\,.
\end{equation}

\begin{table*}
\SetTblrInner{rowsep=0.1cm}
\begin{tblr}{ ||p{5cm}|p{9.5cm}|p{1.2cm}||  }
 \hline
 % \multicolumn{3}{|c|}{Kondo dimer} \\
 \hline
 Energy levels & Eigenstates & Particles\\
 \hline
$\epsilon_0\,=\,-\frac{U}{4}\,-\,\sqrt{\left(\frac{U}{4}\right)^2\,+\,4\,V^2}$ & $\ket{n_{01}}\,=\,\frac{1}{N_{01}}\,\left(\epsilon_0\,\left(\ket{\uparrow,\,\downarrow}\,-\,\ket{\downarrow,\,\uparrow}\right)\,+\,2\,V\,\ket{2,\,0}\,+\,2\,V\,\ket{0,\,2}\right)$ & $n\,=\,2$\\
\hline

$\epsilon_1\,=\,-\frac{U}{4}\,-\,\sqrt{\left(\frac{U}{4}\right)^2\,+\,V^2}$ & $\ket{n_{11}}\,=\,\frac{1}{N_{11}}\,\left(\epsilon_1\,\ket{\uparrow,\,0}\,+\,V\,\ket{0,\,\uparrow}\right)$ & $n\,=\,1$\\
& $\ket{n_{12}}\,=\,\frac{1}{N_{12}}\,\left(\epsilon_1\,\ket{\downarrow,\,0}\,+\,V\,\ket{0,\,\downarrow}\right)$ & $n\,=\,1$\\
& $\ket{n_{13}}\,=\,\frac{1}{N_{13}}\,\left(\epsilon_1\,\ket{\uparrow,\,2}\,+\,V\,\ket{2,\,\uparrow}\right)$ & $n\,=\,3$\\
& $\ket{n_{14}}\,=\,\frac{1}{N_{14}}\,\left(\epsilon_1\,\ket{\downarrow,\,2}\,+\,V\,\ket{2,\,\downarrow}\right)$ & $n\,=\,3$\\
\hline

$\epsilon_2\,=\,-\frac{U}{2}$ & $\ket{n_{21}}\,=\,\frac{1}{N_{21}}\,\left(\ket{\uparrow,\,\downarrow}\,+\,\ket{\downarrow,\,\uparrow}\right)$ & $n\,=\,2$\\
& $\ket{n_{22}}\,=\,\ket{\uparrow,\,\uparrow}$ & $n\,=\,2$\\
& $\ket{n_{23}}\,=\,\ket{\downarrow,\,\downarrow}$ & $n\,=\,2$\\
\hline

$\epsilon_3\,=\,0$ & $\ket{n_{31}}\,=\,\frac{1}{N_{31}}\,\left(\ket{2,\,0}\,-\,\ket{0,\,2}\right)$ & $n\,=\,2$\\
& $\ket{n_{32}}\,=\,\ket{0,\,0}$ & $n\,=\,0$\\
& $\ket{n_{33}}\,=\,\ket{2,\,2}$ & $n\,=\,4$\\
\hline

$\epsilon_4\,=\,-\frac{U}{4}\,+\,\sqrt{\left(\frac{U}{4}\right)^2\,+\,V^2}$ & $\ket{n_{41}}\,=\,\frac{1}{N_{41}}\,\left(\epsilon_4\,\ket{\uparrow,\,0}\,+\,V\,\ket{0,\,\uparrow}\right)$ & $n\,=\,1$\\
& $\ket{n_{42}}\,=\,\frac{1}{N_{42}}\,\left(\epsilon_4\,\ket{\downarrow,\,0}\,+\,V\,\ket{0,\,\downarrow}\right)$ & $n\,=\,1$\\
& $\ket{n_{43}}\,=\,\frac{1}{N_{43}}\,\left(\epsilon_4\,\ket{\uparrow,\,2}\,+\,V\,\ket{2,\,\uparrow}\right)$ & $n\,=\,3$\\
& $\ket{n_{44}}\,=\,\frac{1}{N_{44}}\,\left(\epsilon_4\,\ket{\downarrow,\,2}\,+\,V\,\ket{2,\,\downarrow}\right)$ & $n\,=\,3$\\
\hline

$\epsilon_5\,=\,-\frac{U}{4}\,+\,\sqrt{\left(\frac{U}{4}\right)^2\,+\,4\,V^2}$ & $\ket{n_{51}}\,=\,\frac{1}{N_{51}}\,\left(\epsilon_5\,\left(\ket{\uparrow,\,\downarrow}\,-\,\ket{\downarrow,\,\uparrow}\right)\,+\,2\,V\,\ket{2,\,0}\,+\,2\,V\,\ket{0,\,2}\right)$ & $n\,=\,2$\\
\hline
\hline
\end{tblr}
\centering
\caption{\justifying Energy levels of a Kondo dimer (system with one interacting site hybridized with one non-interacting site) at half-filling. $N_{ii}$ describes a normalization constant for the respective eigenstates.}
\label{tab:Kondo_dimer_energy_levels}
\end{table*} 
\noindent For analytic calculations of spin and charge susceptibilities we use the Lehmann representation. Here, we differentiate transitions between different energy levels and contributions at the same energy. Starting with the spin susceptibility we find the following expression for transitions with varying energies:
\begin{equation}
\begin{split}
    \chi^{\text{spin},\,\epsilon_n\,\neq\,\epsilon_{n'}}_{zz}\,&=\,-\,\frac{1}{Z}\,\sum_{n\,\neq\,n'}\,\frac{e^{-\epsilon_n\,\beta\,}-\,e^{-\epsilon_{n'}\,\beta}}{\epsilon_n\,-\,\epsilon_{n'}}\,\vert{C_{n,\,n'}}\vert{}^2\\
    &=\,-\,\frac{1}{Z}\,e^{-\epsilon_0\,\beta}\,\frac{1\,-\,e^{-\Delta_2\,\beta}}{\Delta_2}\,\left(\vert{C_{0,\,2}}\vert{}^2\,+\,\vert{C_{2,\,0}}\vert{}^2\right)\,-\,\frac{1}{Z}\,e^{-\epsilon_0\,\beta}\,\frac{e^{-\Delta_1\,\beta}\,-\,e^{-\Delta_4\,\beta}}{\Delta_1\,-\,\Delta_4}\,\left(\vert{C_{1,\,4}}\vert{}^2\,+\,\vert{C_{4,\,1}}\vert{}^2\right)\\
    &\,\,\,\,\,\,\,-\,\frac{1}{Z}\,e^{-\epsilon_0\,\beta}\,\frac{e^{-\Delta_2\,\beta}\,-\,e^{-\Delta_5\,\beta}}{\Delta_2\,-\,\Delta_5}\,\left(\vert{C_{2,\,5}}\vert{}^2\,+\,\vert{C_{5,\,2}}\vert{}^2\right)\,,
\end{split}
\end{equation}
with $C_{n,\,n'}\,=\,\sum_i\,\bra{n_{n,\,i}}(\hat{n}_{f\uparrow}\,-\,\hat{n}_{f\downarrow})\ket{n_{n',\,i}}$, where $i$ indicates a sum over the eigenfunctions of the corresponding subspace for the respective energy.
\newpage
\noindent
If the energy levels are equal, we get:
\begin{equation}
\begin{split}
    \chi^{\text{spin},\,\epsilon_n\,=\,\epsilon_{n'}}_{zz}\,&=\,\frac{1}{Z}\,\sum_{n\,=\,n',\,j}\,\beta\,e^{-\epsilon_n\,\beta}\,\vert{C_{n, j}}\vert{}^2\\
    &=\,\frac{\beta}{Z}\,e^{-\epsilon_0\,\beta}\,e^{-\Delta_1\,\beta}\,\left(\vert{C_{1,\,1}}\vert{}^2\,+\,\vert{C_{1,\,2}}\vert{}^2+\,\vert{C_{1,\,3}}\vert{}^2\,+\,\vert{C_{1,\,4}}\vert{}^2\right)\,+\,\frac{\beta}{Z}\,e^{-\epsilon_0\,\beta}\,e^{-\Delta_2\,\beta}\,\left(\vert{C_{2,\,2}}\vert{}^2\,+\,\vert{C_{2,\,3}}\vert{}^2\right)\\
    &\,\,\,\,\,\,\,+\,\frac{\beta}{Z}\,e^{-\epsilon_0\,\beta}\,e^{-\Delta_4\,\beta}\,\left(\vert{C_{4,\,1}}\vert{}^2\,+\,\vert{C_{4,\,2}}\vert{}^2+\,\vert{C_{4,\,3}}\vert{}^2\,+\,\vert{C_{4,\,4}}\vert{}^2\right)\,,
\end{split}
\end{equation}
with $C_{n,\,j}\,=\,\bra{n_{n,\,j}}(\hat{n}_{f\uparrow}\,-\,\hat{n}_{f\downarrow})\ket{n_{n,\,j}}$.
The index $j$ refers to the $j$-th overlap at the same energy level. For $U\,=\,0$ and $V\,=\,2$ the previous expressions yield:
\begin{equation}
    \begin{split}
        \chi^{\text{spin},\,\epsilon_n\,\neq\,\epsilon_{n'}}_{zz}\,&=\,\frac{\frac{1}{2}\,+\,e^{-2\,\beta}\,-\,e^{-6\,\beta}\,-\,\frac{1}{2}\,e^{-8\,\beta}}{2\,\left[1\,+\,4\,e^{-2\,\beta}\,+\,6\,e^{-4\,\beta}\,+\,4\,e^{-6\,\beta}\,+\,e^{-8\,\beta}\right]}\\
        \chi^{\text{spin},\,\epsilon_n\,=\,\epsilon_{n'}}_{zz}\,&=\,\frac{\beta\,\left[e^{-2\,\beta}\,+\,2\,e^{-4\,\beta}\,+\,e^{-6\,\beta}\right]}{1\,+\,4\,e^{-2\,\beta}\,+\,6\,e^{-4\,\beta}\,+\,4\,e^{-6\,\beta}\,+\,e^{-8\,\beta}}
    \end{split}
\end{equation}
and the total spin susceptibility calculates to:
\begin{equation}
    \chi^{\text{spin}}_{zz}\,=\,\chi^{\text{spin},\,\epsilon_n\,\neq\,\epsilon_{n'}}_{zz}\,+\,\chi^{\text{spin},\,\epsilon_n\,=\,\epsilon_{n'}}_{zz}
\end{equation}
Focusing on the charge susceptibility and repeating the previous steps, we find the equations:
\begin{equation}
\begin{split}
    \chi^{\text{charge},\,\epsilon_n\,\neq\,\epsilon_{n'}}\,&=\,-\,\frac{1}{Z}\,\sum_{n\,\neq\,n'}\,\frac{e^{-\epsilon_n\,\beta\,}-\,e^{-\epsilon_{n'}\,\beta}}{\epsilon_n\,-\,\epsilon_{n'}}\,\vert{C_{n,\,n'}}\vert{}^2\\
    &=\,-\,\frac{1}{Z}\,e^{-\epsilon_0\,\beta}\,\frac{1\,-\,e^{-\Delta_3\,\beta}}{\Delta_3}\,\left(\vert{C_{0,\,3}}\vert{}^2\,+\,\vert{C_{3,\,0}}\vert{}^2\right)\,-\,\frac{1}{Z}\,e^{-\epsilon_0\,\beta}\,\frac{e^{-\Delta_1\,\beta}\,-\,e^{-\Delta_4\,\beta}}{\Delta_1\,-\,\Delta_4}\,\left(\vert{C_{1,\,4}}\vert{}^2\,+\,\vert{C_{4,\,1}}\vert{}^2\right)\\
    &\,\,\,\,\,\,\,-\,\frac{1}{Z}\,e^{-\epsilon_0\,\beta}\,\frac{e^{-\Delta_3\,\beta}\,-\,e^{-\Delta_5\,\beta}}{\Delta_3\,-\,\Delta_5}\,\left(\vert{C_{3,\,5}}\vert{}^2\,+\,\vert{C_{5,\,3}}\vert{}^2\right)
\end{split}
\end{equation}
and
\begin{equation}
\begin{split}
    \chi^{\text{charge},\,\epsilon_n\,=\,\epsilon_{n'}}\,&=\,\frac{1}{Z}\,\sum_{n\,=\,n',\,i}\,\beta\,e^{-\epsilon_n\,\beta}\,\vert{C_{n, i}}\vert{}^2\\
    &=\,\frac{\beta}{Z}\,e^{-\epsilon_0\,\beta}\,\vert{C_{0,\,1}}\vert{}^2\,+\,\frac{\beta}{Z}\,e^{-\epsilon_0\,\beta}\,e^{-\Delta_1\,\beta}\,\left(\vert{C_{1,\,1}}\vert{}^2\,+\,\vert{C_{1,\,2}}\vert{}^2+\,\vert{C_{1,\,3}}\vert{}^2+\,\vert{C_{1,\,4}}\vert{}^2\right)\\
    &\,\,\,\,\,\,\,+\,\frac{\beta}{Z}\,e^{-\epsilon_0\,\beta}\,e^{-\Delta_2\,\beta}\,\left(\vert{C_{2,\,1}}\vert{}^2\,+\,\vert{C_{2,\,2}}\vert{}^2\,+\,\vert{C_{2,\,3}}\vert{}^2\right)\,+\,\frac{\beta}{Z}\,e^{-\epsilon_0\,\beta}\,e^{-\Delta_3\,\beta}\,\left(\vert{C_{3,\,1}}\vert{}^2\,+\,\vert{C_{3,\,3}}\vert{}^2\right)\\
    &\,\,\,\,\,\,\,+\,\frac{1}{Z}\,e^{-\epsilon_0\,\beta}\,\beta\,e^{-\Delta_4\,\beta}\,\left(\vert{C_{4,\,1}}\vert{}^2\,+\,\vert{C_{4,\,2}}\vert{}^2+\,\vert{C_{4,\,3}}\vert{}^2\,+\,\vert{C_{4,\,4}}\vert{}^2\right)\,+\,\frac{\beta}{Z}\,e^{-\epsilon_0\,\beta}\,e^{-\Delta_5\,\beta}\,\vert{C_{5,\,1}}\vert{}^2\,.
\end{split}
\end{equation}
In the case of the local charge susceptibility there exists a non-vanishing disconnected part subtracted from the two other contributions in contrast to the local spin susceptibility:
\begin{equation}
\begin{split}
    \chi^{\text{charge},\,\text{discon}}\,&=\,\frac{\beta}{Z^2}\,\left(\sum_{n\,=\,n',\,i}\,e^{-\epsilon_n\,\beta}\,C_{n, i}\right)^2\\
    &=\,\frac{\beta}{Z^2}\,\left[e^{-\epsilon_0\,\beta}\,C_{0,\,1}\,+\,e^{-\epsilon_0\,\beta}\,e^{-\Delta_1\,\beta}\,\left(C_{1,\,1}\,+\,C_{1,\,2}\,+\,C_{1,\,3}\,+\,C_{1,\,4}\right)\right.\\
    &\left.\,\,\,\,\,\,\,+\,e^{-\epsilon_0\,\beta}\,e^{-\Delta_2\,\beta}\,\left(C_{2,\,1}\,+\,C_{2,\,2}\,+\,C_{2,\,3}\right)\,+\,e^{-\epsilon_0\,\beta}\,e^{-\Delta_3\,\beta}\,\left(C_{3,\,1}\,+\,C_{3,\,3}\right)\right.\\
    &\left.\,\,\,\,\,\,\,+\,e^{-\epsilon_0\,\beta}\,e^{-\Delta_4\,\beta}\,\left(C_{4,\,1}\,+\,C_{4,\,2}\,+\,C_{4,\,3}\,+\,C_{4,\,4}\right)\,+\,e^{-\epsilon_0\,\beta}\,e^{-\Delta_5\,\beta}\,C_{5,\,1}\right]^2\,.
\end{split}
\end{equation}
For the charge susceptibility, the $C$ matrix elements are calculated the same way as for the spin susceptibility, but with the expectation values of the charge operator $\hat{n}_{f\uparrow}\,+\,\hat{n}_{f\downarrow}$. 
Here, inserting $U\,=\,0$ and $V\,=\,2$ leads to:
\begin{equation}
    \begin{split}
        \chi^{\text{charge},\,\epsilon_n\,\neq\,\epsilon_{n'}}\,&=\,\frac{\frac{1}{2}\,+\,e^{-2\,\beta}\,-\,e^{-6\,\beta}\,-\,\frac{1}{2}\,e^{-8\,\beta}}{2\,\left[1\,+\,4\,e^{-2\,\beta}\,+\,6\,e^{-4\,\beta}\,+\,4\,e^{-6\,\beta}\,+\,e^{-8\,\beta}\right]}\\
        \chi^{\text{charge},\,\epsilon_n\,=\,\epsilon_{n'}}\,&=\,\frac{\beta\,\left[1\,+\,5\,e^{-2\,\beta}\,+\,8\,e^{-4\,\beta}\,+\,5\,e^{-6\,\beta}\,+\,e^{-8\,\beta}\right]}{1\,+\,4\,e^{-2\,\beta}\,+\,6\,e^{-4\,\beta}\,+\,4\,e^{-6\,\beta}\,+\,e^{-8\,\beta}}\\
        \chi^{\text{charge},\,\text{discon}}\,&=\,\frac{\beta\,\left[1\,+\,4\,e^{-2\,\beta}\,+\,6\,e^{-4\,\beta}\,+\,4\,e^{-6\,\beta}\,+\,e^{-8\,\beta}\right]}{1\,+\,4\,e^{-2\,\beta}\,+\,6\,e^{-4\,\beta}\,+\,4\,e^{-6\,\beta}\,+\,e^{-8\,\beta}}\,=\,\beta
    \end{split}
\end{equation}
and the total charge susceptibility consists of the following combination:
\begin{equation}
    \chi^{\text{charge}}\,=\,\chi^{\text{charge},\,\epsilon_n\,\neq\,\epsilon_{n'}}\,+\,\chi^{\text{charge},\,\epsilon_n\,=\,\epsilon_{n'}}\,-\,\chi^{\text{charge},\,\text{discon}}
\end{equation}
Thus, for $U\,=\,0$ and $V\,=\,2$ the charge and spin susceptibilities match each other.\\ In the following we analyze the limits of small and large temperatures for the local spin susceptibility.
\newpage
\subsubsection{Local spin susceptibility for $T\rightarrow{0}$}
\noindent
In the case $T\,\rightarrow{0}$, the exponential functions vanish and only a constant part in $T$ survives:
\begin{equation}
    \chi^{\text{spin}}_{zz}(T\,\rightarrow{0})\,=\,\chi^{\text{spin},\,\epsilon_n\,\neq\,\epsilon_{n'}}_{zz}(T\,\rightarrow{0})\,=\,\frac{\left(\vert{C_{0,\,2}}\vert{}^2\,+\,\vert{C_{2,\,0}}\vert{}^2\right)}{\Delta_2}\,=\,\frac{4\,\epsilon^2_0}{\epsilon_5\,\left(2\,\epsilon^2_0\,+\,8\,V^2\right)}\,=\,const.\,,
\end{equation}
depending on the interaction $U$, the hybridization $V$ and the eigenenergies summarized in TABLE\,\ref{tab:Kondo_dimer_energy_levels}.

\subsubsection{Large temperature limit}
\noindent
At high temperatures the zeroth order in the expansion around $\beta\,=\,0$ vanishes and only the first order in $\beta$ contributes to the local spin susceptibility:
\begin{equation}
\begin{split}
    \chi^{\text{spin}}_{zz}(T\,\rightarrow{\infty})\,=\,\frac{\beta}{2}\,,
\end{split}
\end{equation}
showing a Curie law for the Kondo dimer at large temperatures.
