# Supplementary material for: Fragility of local moments against hybridization with flat bands
Source: arXiv:2503.14326 source file (2026-08-11)
Supplement: Supplementary file 8 [file Results_out_off_half_filling.tex]

\subsection{Calculations off half-filling}
\,\\
For calculations away from half-filling, we perform QMC calculations with the software package w2dynamics \cite{Wallerberger_2019}. As first step we solve the impurity model at different temperatures for several values of the chemical potential $\mu$ where the desired occupation $n$ is included. Next, we apply an optimization algorithm on the chemical potential minimizing the difference of the occupation to the desired value. We use the chemical potential with appropriate accuracy and compute the local spin susceptibility $\chi^{\text{spin}}_{zz}$ with larger statistics. Thus, by fixing $\alpha$, the interaction $U\,=\,0.575\,\mathcal{D}$ and the occupation on the impurity site, we investigate $\chi^{\text{spin}}_{zz}$ away from half-filling as a function of the temperature $T/\mathcal{D}$. FIG.\,\ref{fig:local_spin_susceptibility_oohf_DOS} shows the behavior for $\alpha\,=\,0$ (a), $\alpha\,=\,0.5$ (b) and $\alpha\,=\,1$ (c) and assumes an occupation of $n\,=\,1.0$, $n\,=\,1.1$ and $n\,=\,1.25$ each. Starting with $\alpha\,=\,0$ the curve of $\chi^{\text{spin}}_{zz}$ approaches the plateau for small temperatures at lower values of $\chi^{\text{spin}}_{zz}$ with larger impurity occupations. This confirms that the screening effect of the bath electrons is supported by the raising probability of double occupation on the impurity site with the increasing occupation. Thus, the spin-$z$ expectation value is lowered, with a direct impact on the local spin susceptibility. For $\alpha\,=\,0.5$ (FIG.\,\ref{fig:local_spin_susceptibility_oohf_DOS} (b)) and $\alpha\,=\,1$ (FIG.\,\ref{fig:local_spin_susceptibility_oohf_DOS} (c)) the effect on $\chi^{\text{spin}}_{zz}$ is less prominent. Here, the curves exhibit a plateau at small temperatures coming from the favored singlet ground state of a Kondo dimer having a larger influence with increasing $\alpha$. This plateau decreases slightly with the impurity occupation. At intermediate temperatures the curves for different fillings and $\alpha\,\neq\,0$ show a maximum independent on the corresponding occupation on the impurity. However, the position of the maxima dependents on $\alpha$. Increasing it, slightly shifts the maximum to larger temperatures.  

\begin{figure*}
    \centering
    \includegraphics[width=0.99\textwidth]{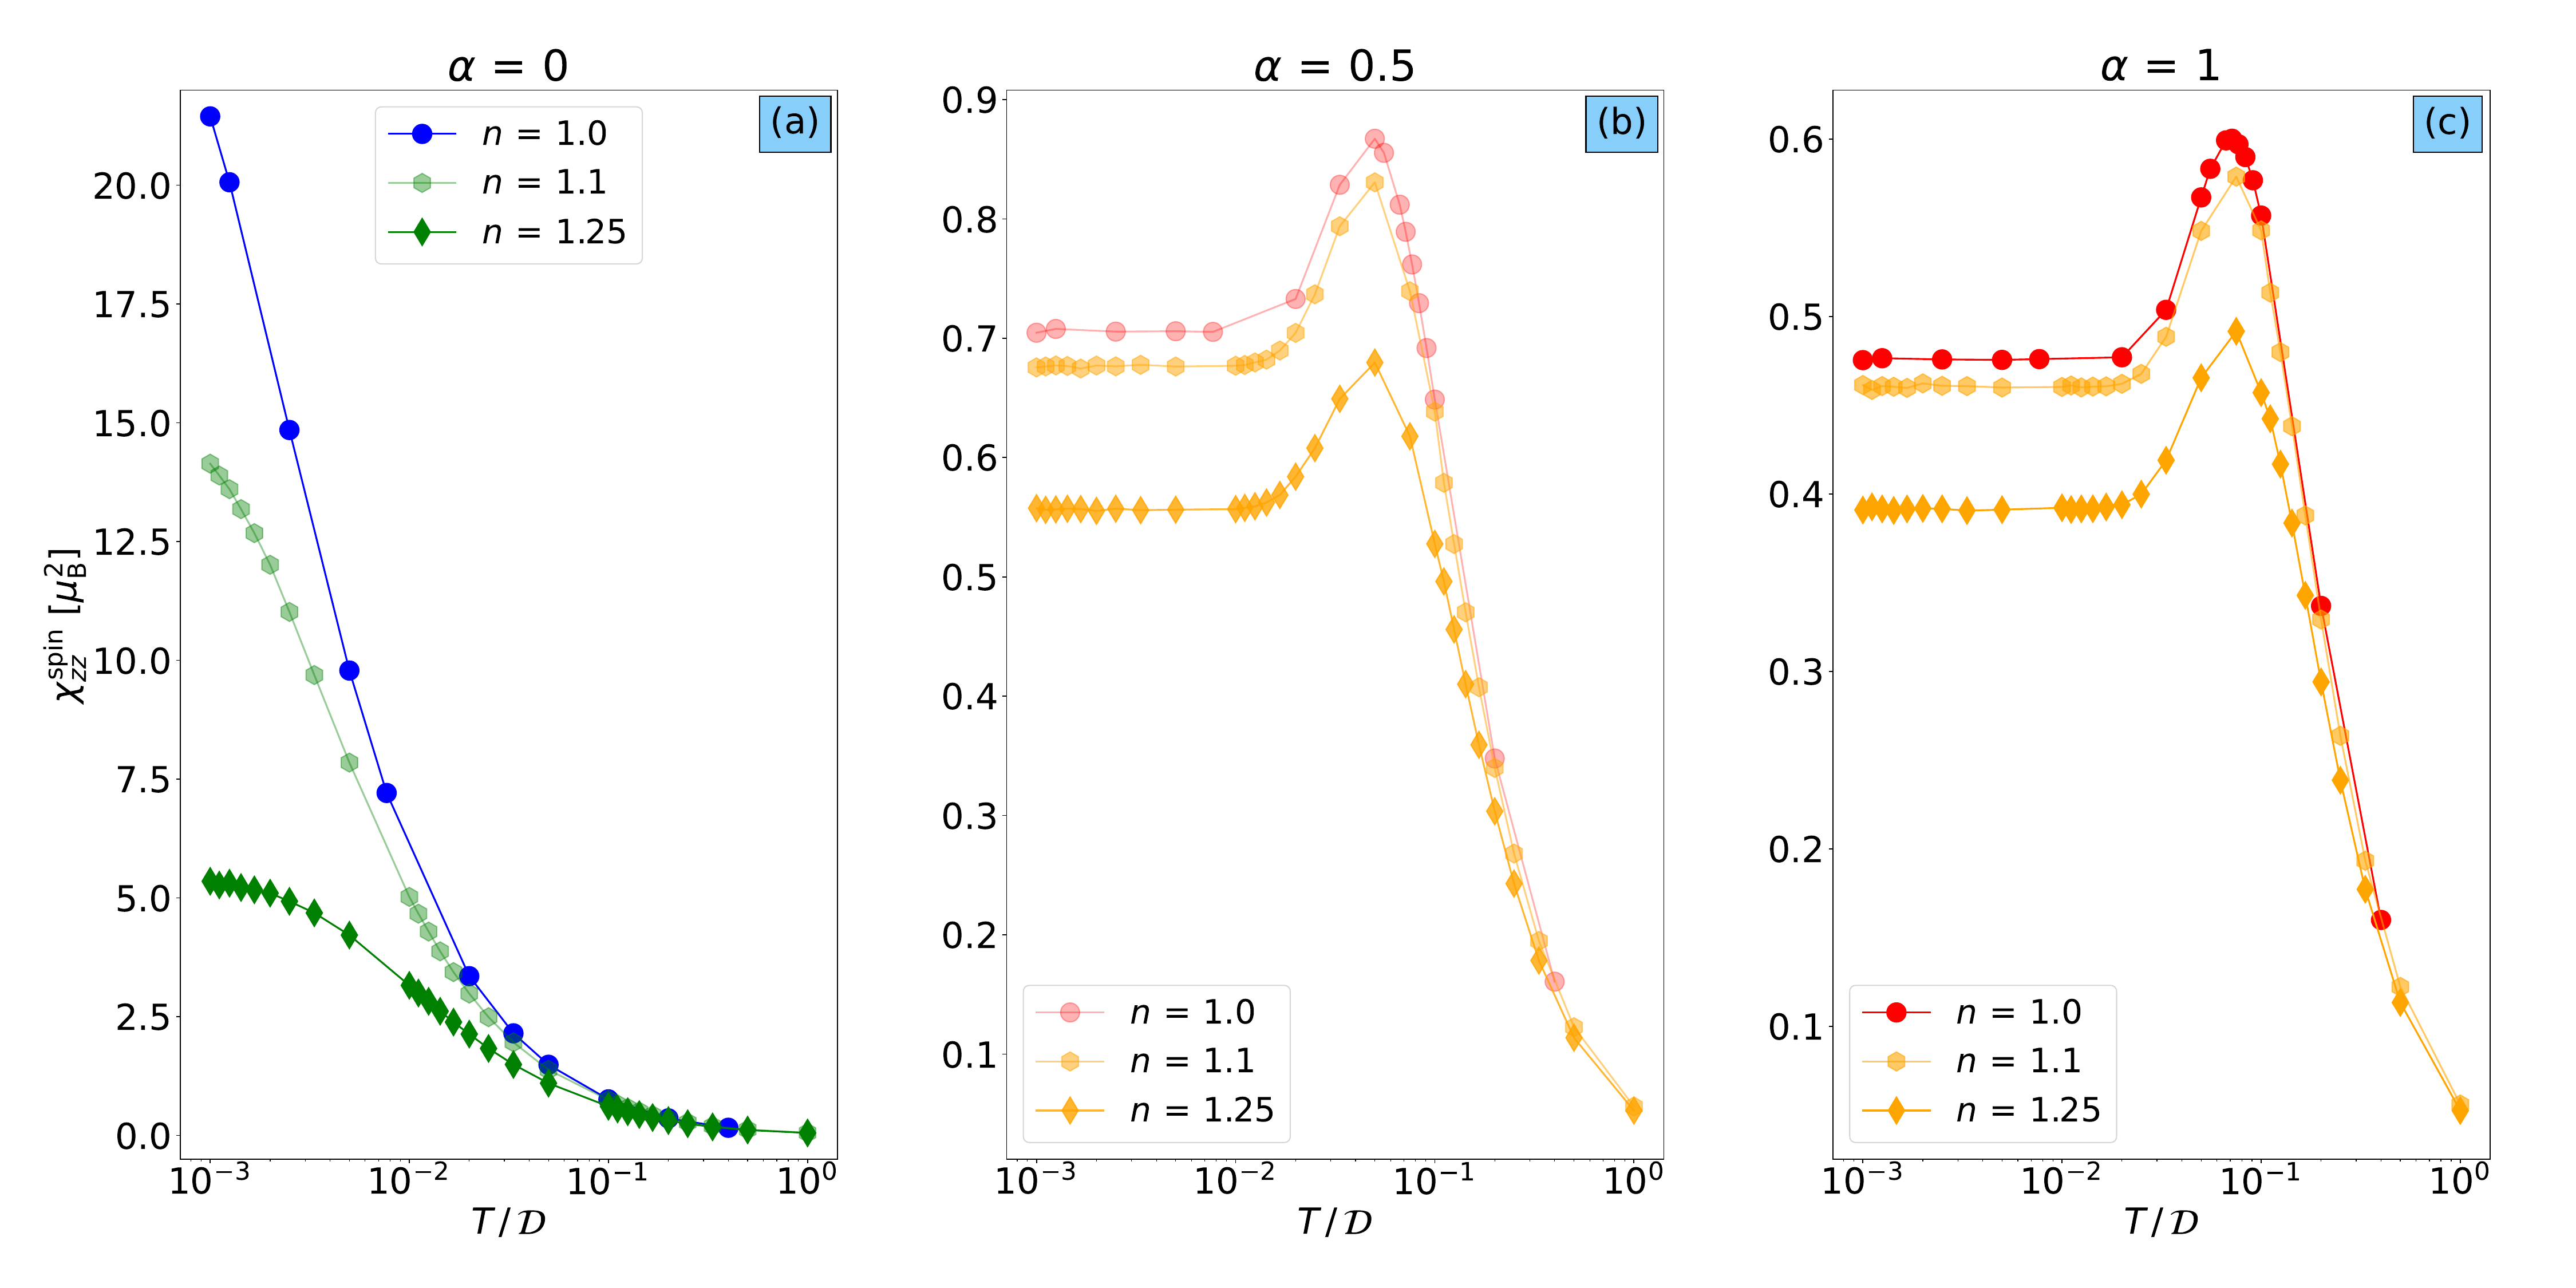}
    \caption{\justifying Local static spin susceptibility $\chi^{\text{spin}}_{zz}$ for several values of $\alpha$ and impurity occupations $n$ at $U\,=\,0.575\,\mathcal{D}$. The weight of the central $\delta$-peak increases from (a) to (c) with $\alpha\,=\,0$, $\alpha\,=\,0.5$ and $\alpha\,=\,1$. At small $\alpha$ the impact of the occupation on the impurity site has a large influence on the value of the plateau at small temperatures. Larger $\alpha$-values show qualitatively similar curves for different occupations. The positions of the maxima of the curves are independent on the respective impurity occupation but they highly depend on the weight $\alpha$.}
    \label{fig:local_spin_susceptibility_oohf_DOS}
\end{figure*}
