# Supplementary material for: Fragility of local moments against hybridization with flat bands
Source: arXiv:2503.14326 source file (2026-08-11)
Supplement: Supplementary file 10 [file System_Hamiltonian_Delta.tex]

\subsection{Anderson impurity model and hybridization function}
\label{sec:system_Hamiltonian_hyb_func_expansion_low_freq}
\noindent We start with the general form of a single-site Anderson impurity model:
\begin{equation}
   \hat{H}\,=\,\sum_{k,\,\sigma}\,\epsilon_{k}\,\hat{c}^{\dagger}_{k\sigma}\,\hat{c}_{k\sigma}\,+\,\sum_{\sigma}\,\epsilon_{f}\,\hat{f}^{\dagger}_{\sigma}\,\hat{f}_{\sigma}\,+\,U\,\hat{n}_{f\uparrow}\,\hat{n}_{f\downarrow}\,+\,\sum_{k,\,\sigma}\,V_k\,\left(\hat{c}^{\dagger}_{k\sigma}\,\hat{f}_{\sigma}\,+\,\hat{f}^{\dagger}_{\sigma}\,\hat{c}_{k\sigma}\right)\,,
\label{eq:general_AIM_Hamiltonian}
\end{equation}
where the first term describes the dispersion $\epsilon_{k}$ of the bath while the second and third terms are the energy level $\epsilon_{f}$ and the interaction $U$ on the impurity site, respectively. The last term denotes the hybridization between the bath and the impurity with the hybridization strength $V_k$, assumed to be constant within the scope of this paper ($V_k\,=\,V$). $\hat{f}^{(\dagger)}_{\sigma}$ and $\hat{c}^{(\dagger)}_{k\sigma}$ are annihilation (creation) operators on the impurity site and in the bath, respectively. The hybridization function is related to the retarded non-interacting Green's function $G_0(\omega)$ via
\begin{equation}
    \Delta(\omega)= \omega + i\eta - \epsilon_f - G^{-1}_0(\omega),
    \label{eq:G0}
\end{equation}
where $\eta$ denotes the symbol used to indicate 0$^+$.\\
For the hybridization function in the main text, we assumed half-filling and particle-hole symmetry, implying in this case $\epsilon_f = -\frac{U}{2}$.
